# Supplementary material for: Statistical methods for partitioning ribbon and globally-distributed flux using data from the Interstellar Boundary Explorer
Source: arXiv:2302.03089 source file (2026-05-22)
Supplement: Supplementary file 1 [file Supplementary_Materials.pdf]

# Supplementary Materials for “Statistical methods for partitioning ribbon and globally-distributed flux using data from the Interstellar Boundary Explorer”

Lauren J. Beesley<sup>\*1,2</sup>, Dave Osthus<sup>2</sup>, Kelly R. Moran<sup>2</sup>, Madeline A. Ausdemore<sup>2</sup>,  
Grant David Meadors<sup>3</sup>, Paul H. Janzen<sup>4</sup>, Eric J. Zirnstein<sup>5</sup>,  
Brian P. Weaver<sup>2</sup>, Daniel B. Reisenfeld<sup>3</sup>

<sup>1</sup>Information Systems & Modeling, Los Alamos National Laboratory

<sup>2</sup>Statistical Sciences, Los Alamos National Laboratory

<sup>3</sup>Intelligence and Space Research, Los Alamos National Laboratory

<sup>4</sup>Physics and Astronomy, University of Montana

<sup>5</sup>Astrophysical Sciences, Princeton University

\*Corresponding Author: [lvandervort@lanl.gov](mailto:lvandervort@lanl.gov)

February 6, 2023

## Contents

|          |                                                                  |           |
|----------|------------------------------------------------------------------|-----------|
| <b>A</b> | <b>Uncertainty estimation</b>                                    | <b>2</b>  |
| <b>B</b> | <b>Ribbon center estimation</b>                                  | <b>6</b>  |
| <b>C</b> | <b>Ribbon separation algorithm</b>                               | <b>8</b>  |
| <b>D</b> | <b>Ribbon Separation in Simulated Data</b>                       | <b>15</b> |
| <b>E</b> | <b>Ribbon Center Estimation in Simulated Data</b>                | <b>20</b> |
| <b>F</b> | <b>Additional results from real IBEX data analysis</b>           | <b>24</b> |
| <b>G</b> | <b>A note on empirical coverage and normality approximations</b> | <b>26</b> |
| <b>H</b> | <b>Choosing mask tuning parameters</b>                           | <b>28</b> |

## A Uncertainty estimation

In this section, we provide more details on our proposed method for estimating ribbon and GDF map standard errors. Recall,  $\mathcal{M}$  denotes the vectorized input map estimates and  $\sigma_{\mathcal{M}}^2$  denotes the corresponding uncertainties, after rotation into the ribbon-centric rotational frame. This input map was estimated using data for the number of ENA detections observed per second within each pixel of the sky.

Let vector  $y$  denote the raw number of ENAs per second “observed” by IBEX for each map pixel, calculated as the ratio of observed ENA counts  $C$  and exposure time  $T$  in seconds. In reality,  $y$  is not *actually* observed by IBEX; instead, a blurred version of  $y$  is observed. Suppose IBEX is pointed at a known latitude and longitude. ENAs detected when IBEX is pointed in that direction may actually originate from a different latitude and longitude near the point direction, where the distribution of origins for ENAs encountered at a given point direction follow a *known* distribution (Osthus et al., 2022). We can approximate  $y$  by taking the raw observed ENA encounters and attributing them to pixels following the known IBEX field of view properties.

For our statistical framework, we will view  $y$  as a theoretical construct and calculate more concrete properties of  $y$  later on. We assume vector element  $C_i$  follows a Poisson distribution with mean  $\mathcal{M}_i T_i$  for each map pixel  $i$ . Approximating the distribution of  $y$  with a normal distribution, we assume  $y_i \sim N(\mathcal{M}_i, \sigma_{iY}^2)$ , where variance  $\sigma_{iY}^2 = \mathcal{M}_i / T_i$  and where  $y_i$ ’s are conditionally independent.

We assume that input map  $\mathcal{M}$  is the sum of a ribbon-only map  $\mathcal{R}$  and GDF-only map  $\mathcal{G}$ . We also assume that  $\mathcal{R}$  and  $\mathcal{G}$  are marginally independent and normally-distributed such that  $\mathcal{R} \sim N(\mu_R, \sigma_{iR}^2)$  and  $\mathcal{G} \sim N(\mu_G, \sigma_{iG}^2)$ . Together, these assumptions imply

$$\begin{pmatrix} \mathcal{G}_i \\ \mathcal{R}_i \\ y_i \end{pmatrix} \sim N \left( \begin{bmatrix} \mu_{iG} \\ \mu_{iR} \\ \mu_{iG} + \mu_{iR} \end{bmatrix}, \begin{bmatrix} \sigma_{iG}^2 & 0 & \sigma_{iG}^2 \\ 0 & \sigma_{iR}^2 & \sigma_{iR}^2 \\ \sigma_{iG}^2 & \sigma_{iR}^2 & \sigma_{iG}^2 + \sigma_{iR}^2 + \sigma_{iY}^2 \end{bmatrix} \right),$$

where  $\mu$  collectively denotes the elements of  $\mu_G$  and  $\mu_R$  and  $\Sigma$  collectively denotes the elements of  $\sigma_G^2$ ,  $\sigma_R^2$ , and  $\sigma_Y^2$ . Using properties of normal distributions, we can express the uncertainties of the separated maps conditional on the observed IBEX data as

$$Var \left( \begin{bmatrix} \mathcal{G}_i \\ \mathcal{R}_i \end{bmatrix} \middle| y_i; \mu, \Sigma \right) = \frac{1}{\sigma_{iG}^2 + \sigma_{iR}^2 + \sigma_{iY}^2} \begin{bmatrix} \sigma_{iG}^2 \{ \sigma_{iR}^2 + \sigma_{iY}^2 \} & -\sigma_{iG}^2 \sigma_{iR}^2 \\ -\sigma_{iG}^2 \sigma_{iR}^2 & \sigma_{iR}^2 \{ \sigma_{iG}^2 + \sigma_{iY}^2 \} \end{bmatrix}.$$

Other terms of interest include:

$$\begin{aligned} Var(\mathcal{G}_i + \mathcal{R}_i | y_i; \mu, \Sigma) &= \sigma_{iY}^2 \frac{\sigma_{iG}^2 + \sigma_{iR}^2}{\sigma_{iG}^2 + \sigma_{iR}^2 + \sigma_{iY}^2} \\ Var(\mathcal{G}_i | \mathcal{R}_i, y_i; \mu, \Sigma) &= \sigma_{iY}^2 \frac{\sigma_{iG}^2}{\sigma_{iG}^2 + \sigma_{iY}^2} \\ Var(y_i | \mathcal{G}_i + \mathcal{R}_i, \mu, \Sigma) &= \sigma_{iY}^2 \end{aligned}$$

Using estimates for each one of these expressions, we can then solve for  $\sigma_{iG}^2$ ,  $\sigma_{iR}^2$ , and  $\sigma_{iY}^2$  using the following relationships:

$$\begin{aligned} \sigma_{iG}^2 &= \frac{Var(\mathcal{G}_i | \mathcal{R}_i, y_i; \mu, \Sigma) \sigma_{iY}^2}{\sigma_{iY}^2 - Var(\mathcal{G}_i | \mathcal{R}_i, y_i; \mu, \Sigma)} \\ \sigma_{iG}^2 + \sigma_{iR}^2 &= \frac{Var(\mathcal{G}_i + \mathcal{R}_i | y_i; \mu, \Sigma) \sigma_{iY}^2}{\sigma_{iY}^2 - Var(\mathcal{G}_i + \mathcal{R}_i | y_i; \mu, \Sigma)} \\ \sigma_{iY}^2 &= Var(y_i | \mathcal{G}_i + \mathcal{R}_i, \mu, \Sigma). \end{aligned}$$

Now, we need to determine how to estimate  $Var(\mathcal{G}_i + \mathcal{R}_i|y_i; \mu, \Sigma)$ ,  $Var(\mathcal{G}_i|\mathcal{R}_i, y_i; \mu, \Sigma)$ , and  $Var(y_i|\mathcal{G}_i + \mathcal{R}_i, \mu, \Sigma)$ . The first uncertainty corresponds to the uncertainty of the total ENA rate map, which is provided by the input map estimation procedure and is treated as known in our analysis.

### A.1 Estimating $Var(\mathcal{G}_i|\mathcal{R}_i, y_i; \mu, \Sigma)$

We have that  $Var(\mathcal{G}_i|\mathcal{R}_i, y_i; \mu, \Sigma) = Var(\mathcal{G}_i|\mathcal{R}_i = 0, y_i; \mu, \Sigma)$ . This corresponds to the expected uncertainty of the GDF in the ribbon mask region, supposing that there was no contribution of ribbon ENAs. Restated, this is the uncertainty of the GDF-only ENA rate, supposing we could perfectly process out the ribbon ENAs ahead of ENA rate estimation.

Uncertainty  $Var(\mathcal{G}_i|\mathcal{R}_i = 0, y_i, \mu, \Sigma)$  can be estimated in two different ways. First, we could apply the GDF estimation methodology (i.e., the GAM and iterative PPR fitting) to the estimated input map uncertainties after masking out the ribbon region. However, the resulting fitted values would not incorporate increased uncertainty due to short observation times for certain narrow parts of the sky. This approach implicitly assumes that the observation times in the masked region are on average similar to observation times for data collected outside the mask region, which may be violated in practice.

Instead, we propose approximating  $Var(\mathcal{G}_i|\mathcal{R}_i = 0, y_i, \mu, \Sigma) \approx \frac{\hat{\mathcal{G}}_i}{\hat{\mathcal{M}}_i} Var(\mathcal{G}_i + \mathcal{R}_i|y_i, \mu, \Sigma)$ , using the estimated GDF map value,  $\hat{\mathcal{G}}_i$ . This expression is motivated by properties of Poisson distributions, where if  $\mathcal{G}_i$  times the observation time  $T_i$  is approximately Poisson, the variance of  $\mathcal{G}_i$  will be approximately  $\mathcal{G}_i/T_i$ . The same is true for  $\mathcal{R}_i$ , where the variance of  $\mathcal{R}_i$  will be approximately  $\mathcal{R}_i/T_i$ . Assuming prior independence of  $\mathcal{R}_i$  and  $\mathcal{G}_i$  given  $T_i$ , the variance of their sum will be approximately  $\mathcal{M}_i/T_i$ , and the uncertainty attributed to the GDF will be approximately proportional to  $\mathcal{G}_i/\mathcal{M}_i$ .

### A.2 Estimating $Var(y_i|\mathcal{G}_i + \mathcal{R}_i, \mu, \Sigma)$

Uncertainty  $Var(y_i|\mathcal{G}_i + \mathcal{R}_i, \mu, \Sigma)$  represents the uncertainty in the raw IBEX ENA rate data for pixel  $i$ , conditional on the estimated map  $\mathcal{M}_i$ . Due to the IBEX field of view, observed ENA encounters measured in a particular look direction can correspond to a known *distribution* of origins near IBEX's point/look direction. We estimate the observed ENA rate for pixel  $i$ ,  $y_i$ , and the observation time attributed to pixel  $i$ ,  $T_i$ , as functions of the blurred observed data as follows. First, we attribute observed follow-up time to each pixel by applying the IBEX field of view point spread function (see Osthus et al. (2022) for details) to each IBEX observation, attributing fractions of time spent looking at a given pixel among the current pixel and neighboring pixels according to the point spread function. We perform a similar operation to estimate the number of background-subtracted ENA encounters to attribute to each pixel. From these, we can estimate corresponding values for  $y_i$  for each pixel. Our goal is then to estimate  $Var(y_i|\mathcal{G}_i + \mathcal{R}_i, \mu, \Sigma) = Var(y_i|\mathcal{M}_i, \sigma_{iY}^2)$ .

Define  $r_i = y_i - \mathcal{M}_i$  to be the residuals between the observed IBEX data and the estimated map  $\mathcal{M}$  from Osthus et al. (2022). Assuming the residuals have mean 0, we have that  $\sigma_{iY}^2 = E(r_i^2|\mathcal{M}_i)$ . Since we only have a single estimate of  $y_i$  for each pixel, we estimate  $\sigma_{iY}^2$  by fitting a spatial model for observed  $r_i^2$ , allowing for borrowing of information on  $r_i^2$  between neighboring pixels. In particular, we fit a projection pursuit regression model with outcome  $r_i^2$ , including  $T_i$  and the spatial location as predictors. The resulting fitted model predictions provide estimates of  $\sigma_{iY}^2$ .

Now, our formulas for estimating  $\sigma_{iG}^2$  and  $\sigma_{iR}^2$  provided above require that  $\sigma_{iY}^2 > Var(\mathcal{G}_i + \mathcal{R}_i|y_i; \mu, \Sigma)$ . However, nothing in the PPR estimation guarantees this relationship. To enforce this ordering, we will update  $\sigma_{iY}^2$  values such that  $\sigma_{iY}^2 \leq Var(\mathcal{G}_i + \mathcal{R}_i|y_i; \mu, \Sigma)$  are assigned  $\sigma_{iY}^2 = \rho Var(\mathcal{G}_i + \mathcal{R}_i|y_i; \mu, \Sigma)$  for some  $\rho > 1$ . As we will show later, smaller values of  $\rho$

correspond to greater uncertainty attributed to ribbon separation. We will return to the choice of  $\rho$  below.

### A.3 Additional uncertainty due to ribbon separation

The total uncertainty captured in the separated maps can be calculated as:

$$Var(\mathcal{G}_i|y_i; \mu, \Sigma) + Var(\mathcal{R}_i|y_i; \mu, \Sigma) = Var(\mathcal{G}_i + \mathcal{R}_i|y_i; \mu, \Sigma) + 2 \frac{\sigma_{iG}^2 \sigma_{iR}^2}{\sigma_{iG}^2 + \sigma_{iR}^2 + \sigma_{iY}^2}.$$

The last term captures uncertainty due to the ribbon separation, which is a function of  $\sigma_{iG}^2$ ,  $\sigma_{iR}^2$ , and  $\sigma_{iY}^2$ . Let function  $s(\Sigma) = 2 \frac{\sigma_{iG}^2 \sigma_{iR}^2}{\sigma_{iG}^2 + \sigma_{iR}^2 + \sigma_{iY}^2}$  denote the additional uncertainty attributed to the ribbon separation. This final term can be re-written as follows:

$$s(\Sigma) = 2\sigma_{iY}^2 \frac{Var(\mathcal{G}_i|\mathcal{R}_i, y_i; \mu, \Sigma)}{[\sigma_{iY}^2 - Var(\mathcal{G}_i|\mathcal{R}_i, y_i; \mu, \Sigma)]^2} [Var(\mathcal{G}_i + \mathcal{R}_i|y_i; \mu, \Sigma) - Var(\mathcal{G}_i|\mathcal{R}_i, y_i; \mu, \Sigma)].$$

Plugging in our proposed estimate of  $Var(\mathcal{G}_i|\mathcal{R}_i, y_i; \mu, \Sigma)$ , we have that

$$s(\Sigma) = 2\sigma_{iY}^2 \frac{\frac{\mathcal{G}_i}{\mathcal{M}_i} \frac{\mathcal{R}_i}{\mathcal{M}_i} Var(\mathcal{G}_i + \mathcal{R}_i|y_i; \mu, \Sigma)^2}{[\sigma_{iY}^2 - \frac{\mathcal{G}_i}{\mathcal{M}_i} Var(\mathcal{G}_i + \mathcal{R}_i|y_i; \mu, \Sigma)]^2}. \quad (Eq. S1)$$

This expression depends on  $Var(\mathcal{G}_i + \mathcal{R}_i|y_i; \mu, \Sigma)$ ,  $\mathcal{G}_i$ ,  $\mathcal{R}_i$ , and  $\sigma_{iY}^2$ .

### A.4 Specifying reasonable $\rho$

Now, consider the bounds on  $\sigma_{iY}^2$ . In order to have a non-zero estimate of  $\sigma_{iG}^2 + \sigma_{iR}^2$ , we need  $\sigma_{iY}^2 > Var(\mathcal{G}_i + \mathcal{R}_i|y_i; \mu, \Sigma)$ . We also observe that Eq. S1 increases as  $\sigma_{iY}^2$  approaches  $Var(\mathcal{G}_i + \mathcal{R}_i|y_i; \mu, \Sigma)$ . Therefore, we can enforce upper bounds on total ribbon separation uncertainty  $s(\Sigma)$  based on how close we allow  $\sigma_{iY}^2$  to approach  $Var(\mathcal{G}_i + \mathcal{R}_i|y_i; \mu, \Sigma)$ . As suggested previously, suppose we posit a lower bound to  $\sigma_{iY}^2$  such that  $\sigma_{iY}^2 \geq \rho Var(\mathcal{G}_i + \mathcal{R}_i|y_i; \mu, \Sigma)$ . Then, the chosen value of  $\rho$  will control the upper bounds that can be attained by  $s(\Sigma)$ .

Suppose we want to restrict the ribbon separation uncertainty  $s(\Sigma)$  to be no greater than  $\omega Var(\mathcal{G}_i + \mathcal{R}_i|y_i; \mu, \Sigma)$  for some  $\omega > 0$ . For example, it may be reasonable to require the additional uncertainty added due to ribbon separation cannot be larger than two times the uncertainty of the input map (i.e.,  $\omega = 2$ ). For a fixed  $\omega$  and defining  $p_i = \frac{\mathcal{R}_i}{\mathcal{M}_i}$ , we can obtain a bound on  $\rho$  using Eq. S1 as follows:

$$\begin{aligned} \omega &= \frac{s(\Sigma)}{Var(\mathcal{G}_i + \mathcal{R}_i|y_i; \mu, \Sigma)} = 2\sigma_{iY}^2 \frac{(1 - p_i)p_i Var(\mathcal{G}_i + \mathcal{R}_i|y_i; \mu, \Sigma)}{[\sigma_{iY}^2 - (1 - p_i)Var(\mathcal{G}_i + \mathcal{R}_i|y_i; \mu, \Sigma)]^2} \\ &\leq 2\rho Var(\mathcal{G}_i + \mathcal{R}_i|y_i; \mu, \Sigma) \frac{(1 - p_i)p_i Var(\mathcal{G}_i + \mathcal{R}_i|y_i; \mu, \Sigma)}{[\rho Var(\mathcal{G}_i + \mathcal{R}_i|y_i; \mu, \Sigma) - (1 - p_i)Var(\mathcal{G}_i + \mathcal{R}_i|y_i; \mu, \Sigma)]^2} \\ &= 2\rho \frac{(1 - p_i)p_i}{[\rho - (1 - p_i)]^2}. \end{aligned}$$

This final expression is maximized in  $p_i$  for  $p_i = \frac{\rho-1}{2\rho-1}$ . Plugging this into the final expression, we obtain  $\omega \leq \frac{1}{2(\rho-1)}$ . This provides an upper bound for the maximum possible attainable  $\omega$ , which can guide choices of  $\rho$ . We propose using  $\rho = 1.5$ , which corresponds to  $\omega = 1$ . Restated,  $\rho = 1.5$  restricts the *additional* uncertainty due to ribbon separation to be no more than the uncertainty of the input total ENA rate map. By allowing the uncertainty due to the ribbon separation to be fairly large if supported by the data, we can accommodate the scenario where there is a lot of data for estimating the total ENA rate in a given pixel but less information in the data regarding the relative contributions of the GDF and ribbon to this total ENA rate.

## A.5 A bootstrap alternative for variance estimation

The above variance estimation strategy is appealing in that it is simple and fast to implement. Additionally, it does not require the entire covariance matrix for the total ENA rate map estimates, which for a 2-degree ENA map can be about 3 gigabytes each to store. Two key limitations, however, are its reliance on normal distribution approximations (including for confidence interval construction) and the need to estimate  $\sigma_{iY}^2$  and implement ad hoc thresholding.

An alternative variance estimation strategy is to apply bootstrap methods. In particular, suppose we have access to the raw data used to generate the total ENA rate map rather than just the total ENA rate map and its pixel-level uncertainty estimates. In this case, we can apply the methods in Osthus et al. (2022) to bootstrap samples of the raw IBEX data to generate many total ENA rate maps. For each total ENA rate map, we can then apply the proposed ribbon separation method to obtain estimates of the ribbon and GDF map partitioning. Uncertainty in the pixel-level ENA rate estimates for each of the ribbon and GDF maps across bootstrap samples would then capture uncertainty in the total ENA rate map and uncertainty due to the ribbon separation. Compared to the proposed variance estimation strategy, the bootstrap strategy is much more computationally expensive; however, this computation can be performed in parallel across bootstrap samples. The resulting uncertainty estimates and confidence intervals (obtained using quantiles of the bootstrap map estimates), would no longer rely on the normal distribution approximations or the ad hoc thresholding. The current paper does not implement this variance estimation procedure, but we plan to implement this proposed bootstrap variance estimation method into a cohesive IBEX data analysis pipeline in the future.

## B Ribbon center estimation

In this section, we provide a step-by-step explanation of the proposed ribbon center estimation methodology. Prior to estimation, we fix a working rotational frame (i.e., a working initial ribbon center estimate) in which the ribbon center sits at the North pole. We also suppose we have an input ENA rate map and corresponding uncertainties. The ribbon center algorithm can then be iterated to substantially reduce sensitivity to the initial assumed location of the ribbon center.

### Estimate ENA rate covariance matrix:

1. Rotate data into the working ribbon-centric rotational frame
2. Exclude azimuthal angles between 126 and 192, following Funsten et al. (2013). The goal of that exclusion is to narrow our focus to where the ribbon is more reliably identified.
3. Exclude polar angles less than 80 and greater than 130, to narrow focus to the region likely containing the ribbon peaks. This assumption can be weakened in practice, perhaps at the expense of ribbon peak estimation stability.
4. Each map's observed ENA rates can then be recast in terms of a rectangular matrix with polar angle bins as rows and azimuthal angle bins as columns. Let  $\rho_K$  be a matrix containing estimated Spearman correlations between pairs of polar angle bin rows and let  $\rho_J$  be a matrix with estimated Spearman correlations between pairs of azimuthal angle columns.
5. Consider this same data matrix in terms of a stacked dataset, where each row corresponds to an azimuthal angle x polar angle combination, where rows are ordered first by azimuthal angle and then polar angle within each azimuthal angle. We estimate the full correlation matrix between pairs of pixels as  $\rho = \rho_J \otimes \rho_K$ , where  $\otimes$  denotes a Kronecker product.
6. Letting  $\sigma_M$  denote the standard errors of the estimated input map ENA rates. Then, we estimate the full covariance matrix as  $\Sigma = \text{diag}(\sigma_M) \times \rho \times \text{diag}(\sigma_M)$ , where  $\text{diag}(\sigma_M)$  is a diagonal matrix with vector  $\sigma_M$  along the diagonal.

### Obtain draws of ribbon center:

1. Draw a new ENA rate map from a multivariate normal distribution with mean equal to the input ENA rate map values (subsetted to polar angles 80-130 and excluding azimuthal 126-192) and covariance matrix  $\Sigma$ .
2. Estimate the ribbon peak location for each azimuthal sector using the method in **Supp. Section C**.
3. Estimate the best fitting plane through these peak points using singular value decomposition as described in Blum et al. (2015). Project the peak points onto the best fitting plane using Rodrigues vector rotation (Dai, 2015).
4. Fit an ellipse using the *fitConic* package in R (Fitzgibbon et al., 1999). Then, estimate the covariance matrix associated with the ribbon center Cartesian coordinates in the plane using leave-one-out jackknife estimation (Efron and Stein, 1981). Finally, draw Cartesian coordinates for the ellipse center in the plane from a bivariate normal distribution and calculate the corresponding latitude and longitude of this ribbon center value in the original rotational frame of  $\mathcal{D}$ . This is calculated based on the intersection between a unit sphere and the normal/perpendicular line passing through the drawn ellipse center.
5. Rotate the estimated ribbon center locations into the ecliptic rotational frame.

6. Repeat the above steps for many drawn ENA rate maps to obtain a pseudo-posterior sample of ribbon center estimates in ecliptic coordinates.

For comparison, we also implemented the method in Funsten et al. (2013) using our best effort to reproduce the method proposed in the paper. Key differences between the proposed methods are that the method in Funsten et al. (2013) does not use draws of the input ENA rate maps, it estimates the ellipse in the working rotational frame rather than the frame defined by the best-fitting plane, and it estimates ribbon peaks assuming a Gaussian profile shape for the ribbon cross-sections within each azimuthal angle bin.

## C Ribbon separation algorithm

In this section, we provide a step-by-step explanation of the proposed ribbon separation methodology. Prior to implementing this algorithm, we assume that we have rotated the input map  $\mathcal{D}$  and corresponding uncertainties  $\sigma_D^2$  into the rotational frame defined by the estimated ribbon center. Using this input map, we perform the following steps in order.

### Ribbon peak estimation:

1. For each azimuthal sector, apply cubic interpolation to estimate the input map ENA rate for a fine grid of polar angles (e.g., 0.01 degree intervals). Identify the polar angle with the highest predicted ENA rate.
2. Treating the estimated peaks across azimuthal angles as a time series, filter out outliers in the ribbon peak estimates using the method in the *tsoutliers* function in the R package *forecast* (Hyndman and Khandakar, 2008).
3. Further control outliers and stabilize peak estimates across azimuthal angles by applying local regression smoothing, incorporating wrapping of the sphere across azimuthal angles by fitting to an augmented dataset containing three copies of the estimated ribbon peaks with modified azimuthal angles.

**Figure C1:** Example map with estimated peaks (gray line). Low ENA rates/intensities are shown with black/blue and high ENA intensities are shown with red/magenta.

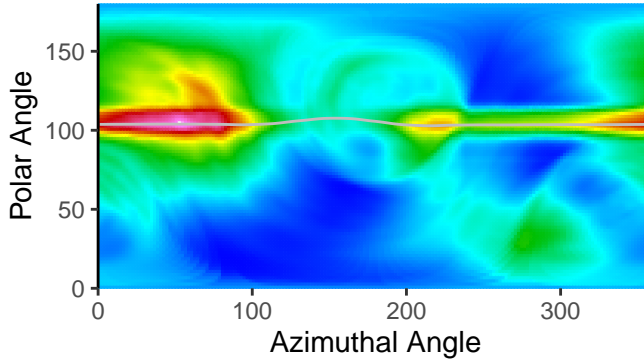

### Ribbon mask identification:

1. Re-organize the data heatmap with longitude on the x-axis and distance from peak (rounded into pixels) on the y-axis
2. Apply local polynomial regression to soften gradients across azimuthal angles

**Figure C2:** Example map with y-axis reorganized relative to distance from ribbon peaks, after local polynomial regression smoothing. Low ENA rates/intensities are shown with black/blue and high ENA intensities are shown with red/magenta.

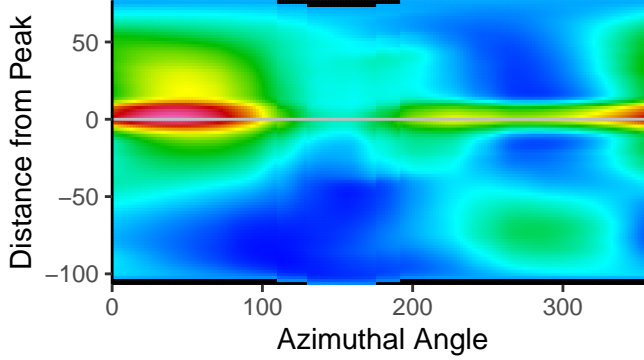

3. Apply the Sobel operator to estimate the “edginess” of each pixel
4. Exclude all pixels with distance from peak  $> v$  degrees (e.g., 30). This ribbon distance/bound can be treated as a sensitivity parameter, as described in **Supp. Section H**.

**Figure C3:** Example Sobel gradient estimates, zooming in to the 30 degrees above and below the ribbon peak. Low gradients are shown with white/light yellow and high gradients are shown with red/black.

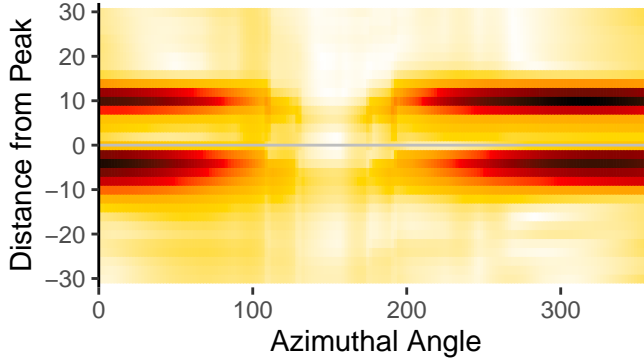

5. Exclude all remaining pixels with Sobel gradients below the  $u^{th}$  (e.g., 75th) quantile. In practice, this quantile can be treated as a sensitivity parameter, as described in **Supp. Section H**.
6. Among the remaining included pixels, define the mask to correspond to the most extreme distances above and below the ribbon peak across all azimuthal sectors
7. A two pixel buffer is then added to the mask to ensure that the entire ribbon is contained within it

**Figure C4:** Example Sobel gradient estimates, after excluding the 75% lowest values. Low gradients are shown with white/light yellow and high gradients are shown with red/black.

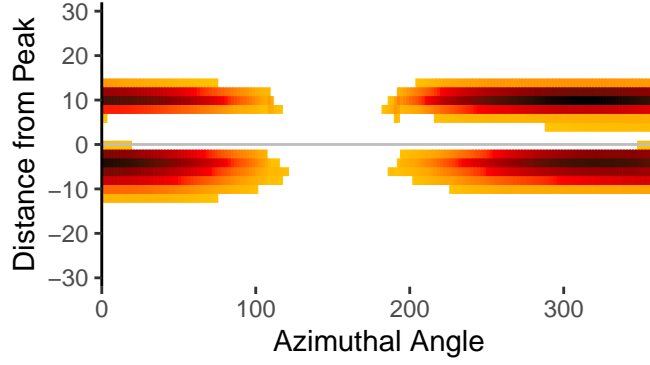

8. The masked pixels are then mapped to their original polar/azimuthal coordinate to define a band of masked pixels on either side of the azimuthal angle-varying ribbon peaks.

**Figure C5:** Original ENA rate map with ENA mask shown as the horizontal gray banded region.

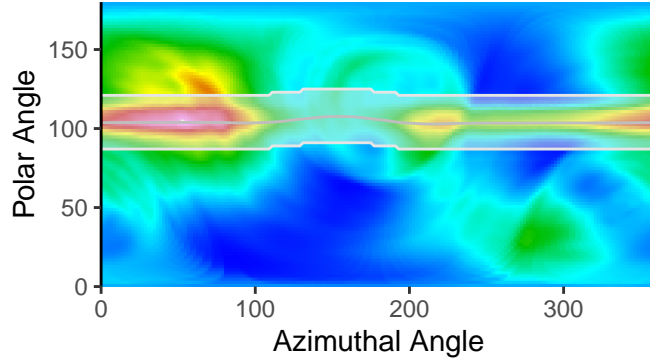

### Initial GDF mapping:

1. Excluding the ribbon mask, fit a generalized additive model (GAM) using the R package *mgcv* and the following pseudo-code:

```
# Fit generalized additive model on input map ENA rates
mgcv::gam(input_ena_rate ~ s(latitude, longitude, bs = "sos", m = 4),
          data=data_excluding_mask, family = gaussian(link = 'log'))
```

**Figure C6:** GDF estimate from fitting GAM to ENA rates, excluding ribbon region. Horizontal gray banded region denotes the ribbon mask.

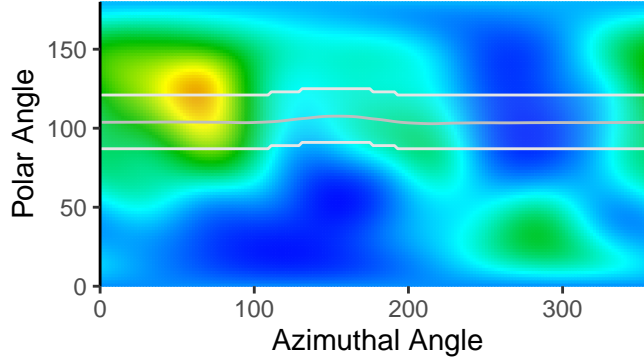

2. Convert latitude/longitudes into cartesian coordinates, x/y/z.
3. For projection pursuit regression (PPR) on the estimation residuals using the following pseudo-code method:

```
# Fit projection pursuit regression on residuals
ppr(resid_gdf ~ x + y + z, nterms = 100, data = data_excluding_mask)
```

4. Perform a second iteration of PPR on the estimation residuals for predicted GDF map, after incorporating the fitted residuals from the first PPR:

```
# Fit second projection pursuit regression on updated residuals
ppr(resid_gdf_ppr ~ x + y + z, nterms = 100, data = data_excluding_mask,
    weights = abs(resid_gdf_ppr))
```

5. The initial GDF map estimate is the GAM prediction plus the first PPR prediction plus the second PPR prediction. GDF map values outside the ribbon mask are set to equal the input map ENA rates, negative GDF map values are thresholded to zero, and GDF map estimates in the mask region greater than the input map value are set equal to the input map value.

**Figure C7:** Initial GDF estimate obtained from GAM and two PPR fits, excluding ribbon region. Horizontal gray banded region denotes the ribbon mask.

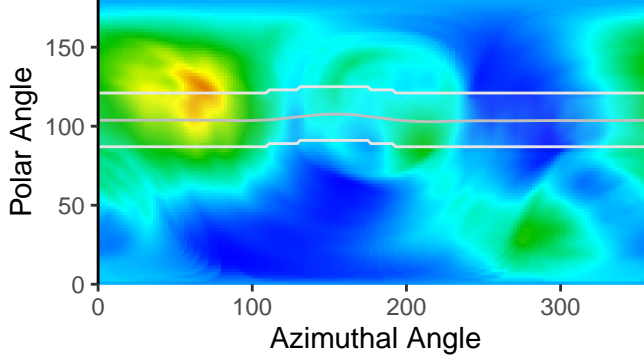

#### Fitted ribbon mapping:

1. Obtain the initial ribbon map estimate by subtracting the initial GDF map estimate from the observed total ENA rate data for all pixels. Off the ribbon mask, this initial ribbon map estimate will exactly equal zero. On the ribbon mask, it will be exactly zero or greater than zero
2. Using the initial ribbon map, re-estimate the ribbon peaks.

**Figure C8:** Initial ribbon map estimate, zooming in on the ribbon region. Ribbon peak estimates are shown with a horizontal wavy line, as are the edges of the ribbon mask region.

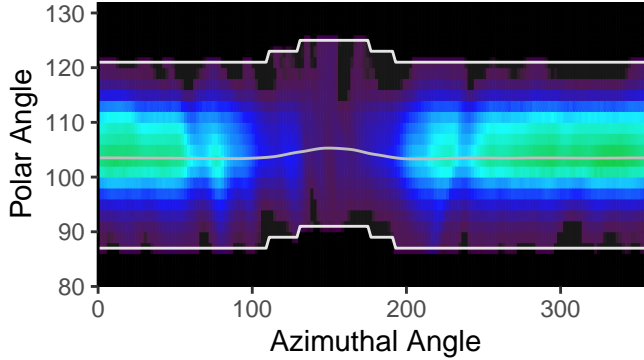

3. For each azimuthal sector, divide out the estimated height of the ribbon peak for that sector.
4. Pre-process out high-intensity values (profile proportion  $> 1.25$ ) far from the ribbon peaks ( $> 4$  degrees away) by setting their ribbon profile values to NA. These values are expected to be associated with non-ribbon ENAs.
5. Then, fit the following generalized additive model to 1-ribbon profile intensity, as described with the following pseudocode. The reason behind using one minus the ribbon profile intensity is to simplify use of existing software and help the predicted ENA rates match up better above and below the ribbon peaks. To enforce a ribbon that is non-increasing from the peak, we use I-splines (Ramsay, 1988), which are integrated non-negative polynomial splines (M-splines), as implemented by the R package *splines2*. To allow for very flexible ribbon profiles, we use 10 knots for this profile fit. Variation across azimuthal angles

**Figure C9:** Initial ribbon profile map estimate, zooming in on the ribbon region. Ribbon peak estimates are shown with a horizontal wavy line, as are the edges of the ribbon mask region. White pixels indicate low ribbon ENA rates, while darker/black pixels indicate higher ribbon ENA rates, relative to the peak heights.

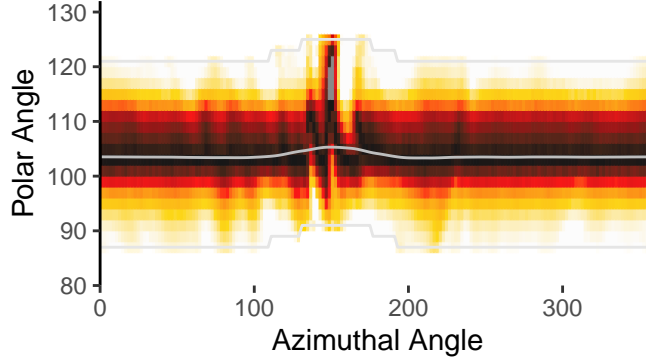

was modeled using periodic B-splines as implemented in the R package *pbs*, which also allowed us to incorporate spatial wrapping across azimuthal sectors by imposing 360-degree periodicity. Twelve basis functions were used for the periodic B-splines, which allows the ribbon profile shape to vary on the order of 30 degrees. Using this model fit, we obtained fitted ribbon profile estimates.

```
# Fit generalized additive model for ribbon
mgcv::gam(one_minus_ribbon_profile_rate)~
  iSpline(dist_above_peaks, knots = list_of_10_knots, intercept = F)*
  pbs(x=azimuthal_discrete, df = 12, intercept = T)+
  iSpline(dist_below_peaks, knots = list_of_10_knots, intercept = F)*
  pbs(x=azimuthal_discrete, df = 12, intercept = T),
  data = data_including_mask, select = T)
```

**Figure C10:** Fitted ribbon profile map estimate, zooming in on the ribbon region. Ribbon peak estimates are shown with a horizontal wavy line, as are the edges of the ribbon mask region. White pixels indicate low ribbon ENA rates, while darker/black pixels indicate higher ribbon ENA rates, relative to the peak heights.

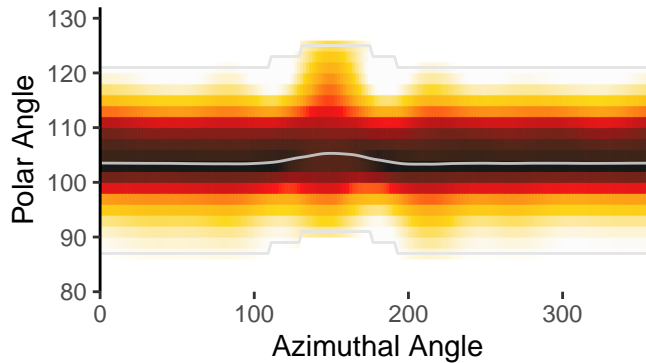

6. We then multiply the fitted profile values within each azimuthal sector with the peak ENA rates divided out earlier to obtain an estimate for the fitted ribbon map.

**Re-estimated GDF and ribbon maps:**

**Figure C11:** Fitted ribbon map estimate, zooming in on the ribbon region. Ribbon peak estimates are shown with a horizontal wavy line, as are the edges of the ribbon mask region.

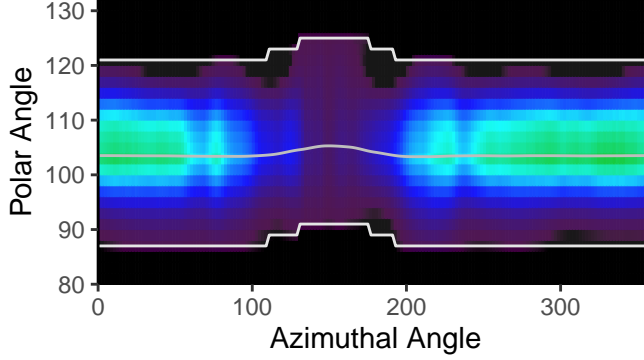

1. Subtracting the fitted ribbon map from the input total ENA rate data, we obtain a rough GDF map estimate. Using this rough map as inputs, we apply the GDF map estimation methods (i.e., GAM and PPR fitting). Unlike before, however, we do not exclude the ribbon mask region. This results in the final GDF map estimate, where pixels outside the ribbon mask region are set exactly equal to the input map ENA rate and where pixels with estimated GDF map values above the total ENA rate have their GDF map value re-assigned to equal the total ENA rate.
2. The final ribbon mask estimate is obtained by subtracting the final GDF map estimate from the input total ENA rate map. This map value will be exactly zero outside the ribbon mask region.

**Figure C12:** Final GDF and ribbon map estimates.

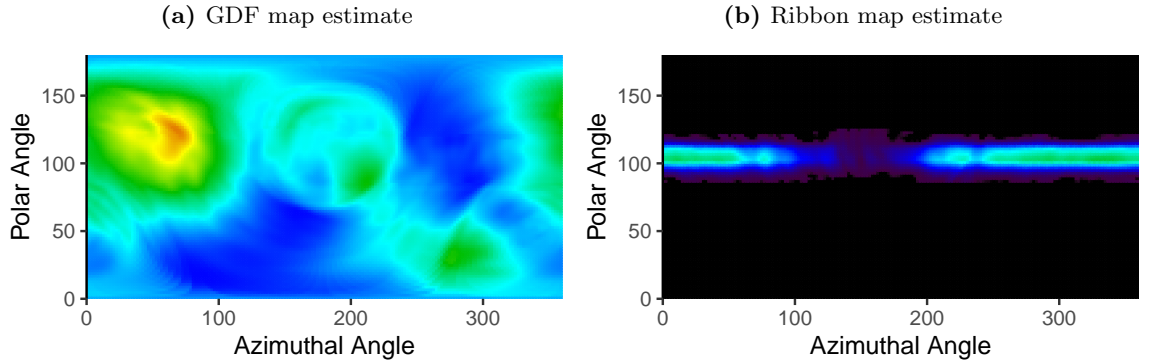

## D Ribbon Separation in Simulated Data

In this section, we provide additional visualization and evaluation of the proposed ribbon separation method in simulated data.

First, we visually inspect the separated ribbon-only and GDF-only maps for “ideal” simulated data inputs. **Supp. Figure D1a** provides the separated maps obtained using the proposed method for ideal input maps, and results for estimated input maps are shown in **Supp. Figure D1b**. Little or no banding can be seen in the GDF-only maps for scenarios S1/S2, which is one indicator that the ribbon separation method performed well. Some ribbon separation artifacts can be seen for scenario S3, where residual banding can be seen in the GDF-only map estimates. Importantly, scenario S3 is unrealistic and intended to help characterize the limitations of the proposed methods. As shown in **Supp. Figure D2**, the ribbon separation method in Reisenfeld et al. (2021) produces substantial banding in all settings (beyond what is seen in any separation using the proposed method).

We provide a direct comparison of the posterior GDF map uncertainties from the proposed methods and the method in Reisenfeld et al. (2021) in **Supp. Figure D3**. Unlike existing methods, the proposed method directly incorporates uncertainty due to the ribbon separation, resulting in slightly increased uncertainty estimates along the ribbon. This results in GDF and ribbon maps that have total uncertainty *greater* than the uncertainty of the input GDF+ribbon map (**Supp. Figure D4**). In contrast, Reisenfeld et al. (2021) does not propagate ribbon separation uncertainty into the uncertainty estimates for the separated maps.

In addition to obtaining accurate map partitions, we are also interested in evaluating the estimated shapes of the ribbon profiles. **Supp. Figure D5** shows the estimated skewness of estimated ribbon map profiles for each azimuthal sector and compares results using the proposed method and the method in Reisenfeld et al. (2021) to the simulation truths. Unsurprisingly, the method in Reisenfeld et al. (2021) produces ribbon maps with near-zero skewness, as a consequence of the Gaussian profile assumptions used in separation. In contrast, the proposed methods can capture non-zero skewness. However, the proposed method still results in skewness that is conservative (i.e., too close to zero). This is particularly true for estimated input maps, since these maps often exhibit weaker ribbon skewness due to the map estimation procedure.

We compare the estimated ribbon widths between methods in **Supp. Figure D6**. We found that the proposed method resulted in more accurate ribbon width estimates than the method in Reisenfeld et al. (2021) on average, and this difference is particularly notable for scenario S2.

**Figure D1:** Map separations for (a) ideal input maps and (2) estimated input maps across different simulation scenarios using the proposed method

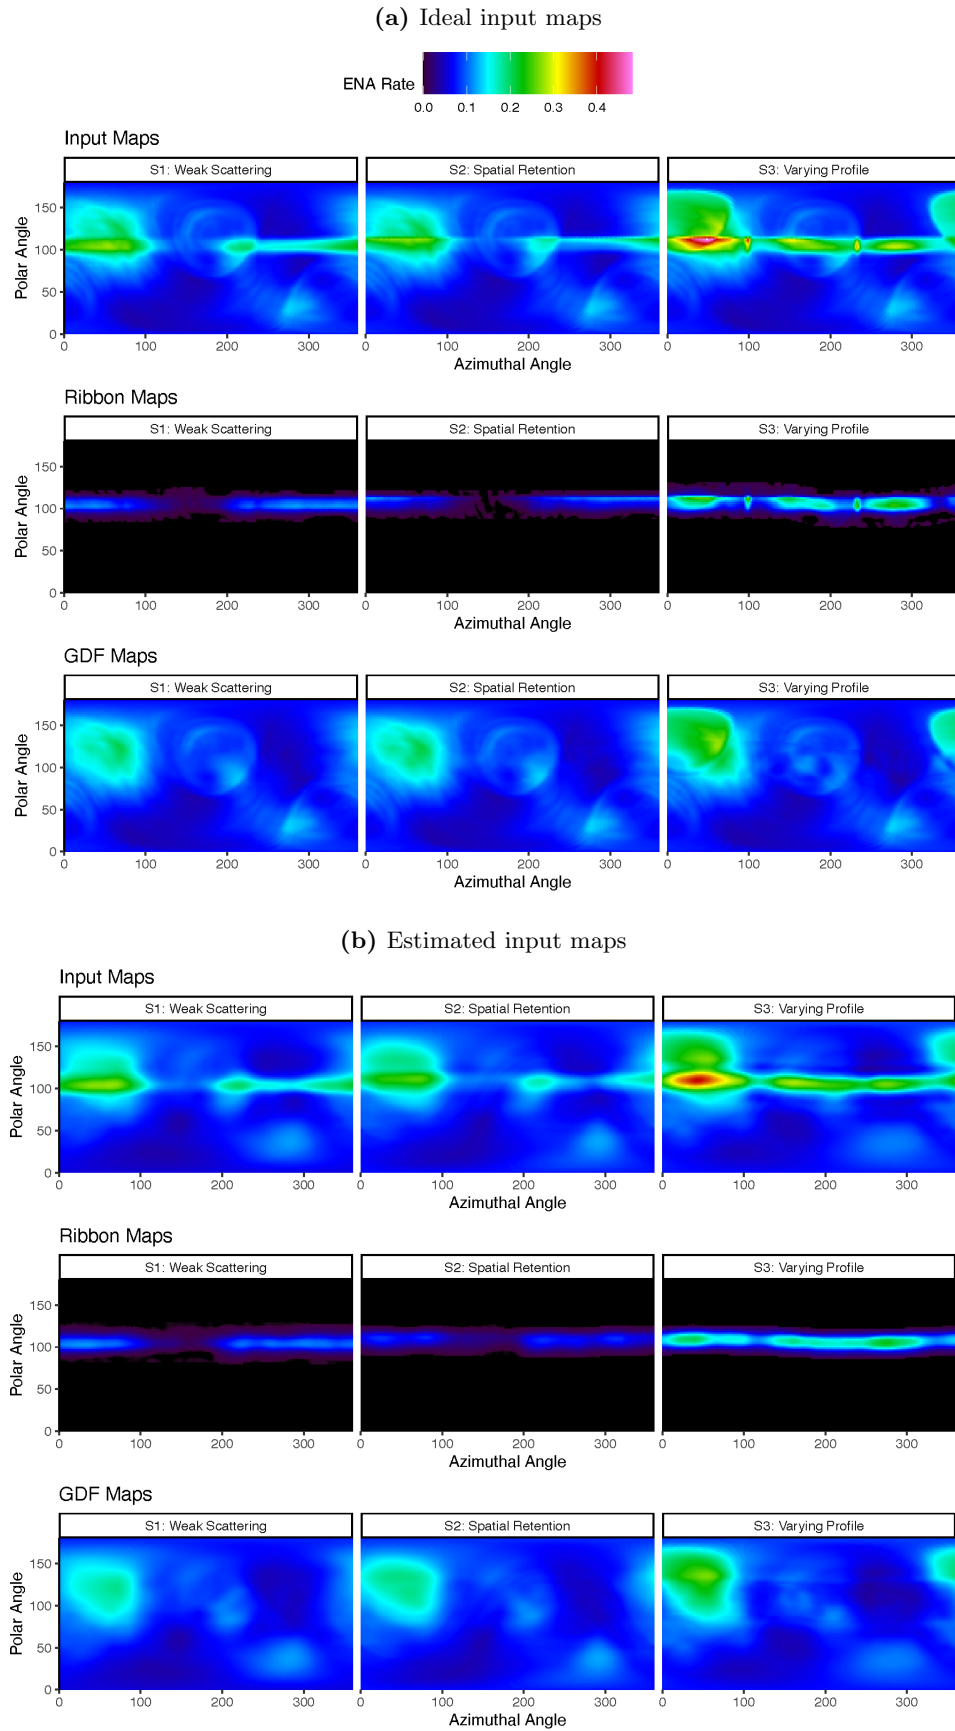

**Figure D2:** Map separations for ideal input maps using the method in Reisenfeld et al. (2021)

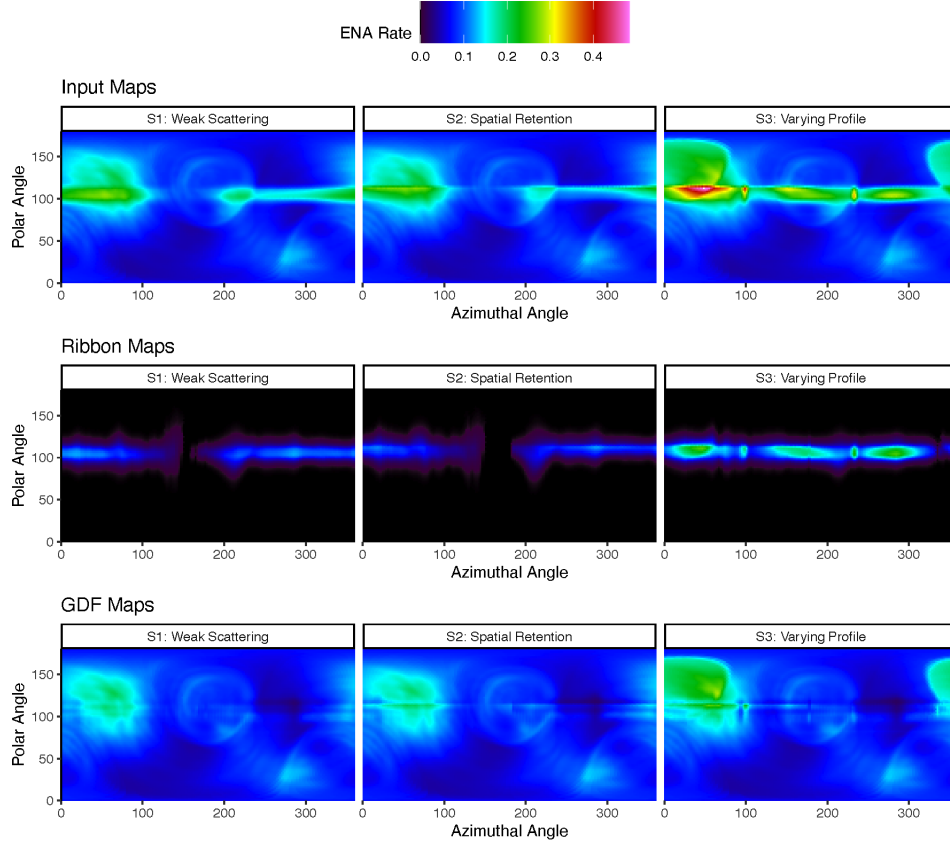

**Figure D3:** Standard errors in separated GDF maps obtained using the methods proposed in Supp. Section A and using the approach in Reisenfeld et al. (2021).

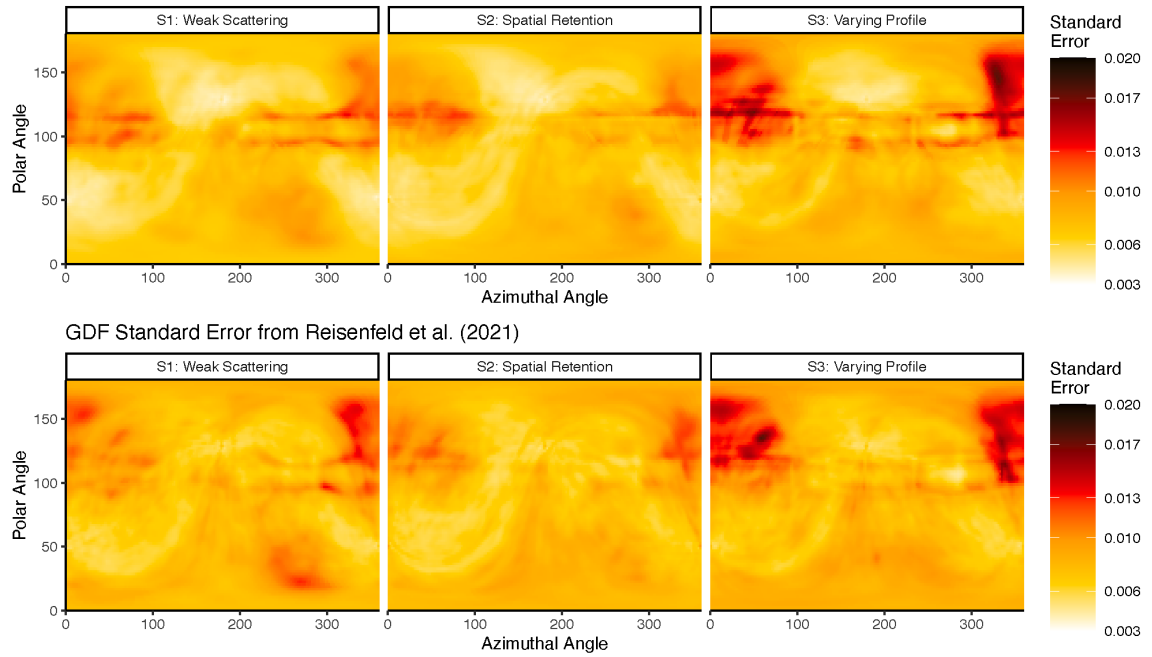

**Figure D4:** Total uncertainty for separated GDF and ribbon maps (a) compared to uncertainty of input GDF+ribbon maps (b) using the proposed methods. The difference between uncertainties in (a) and (b) is shown in (c). Results are shown for polar angles between 80 and 130, which contain the full ribbon in the simulated data.

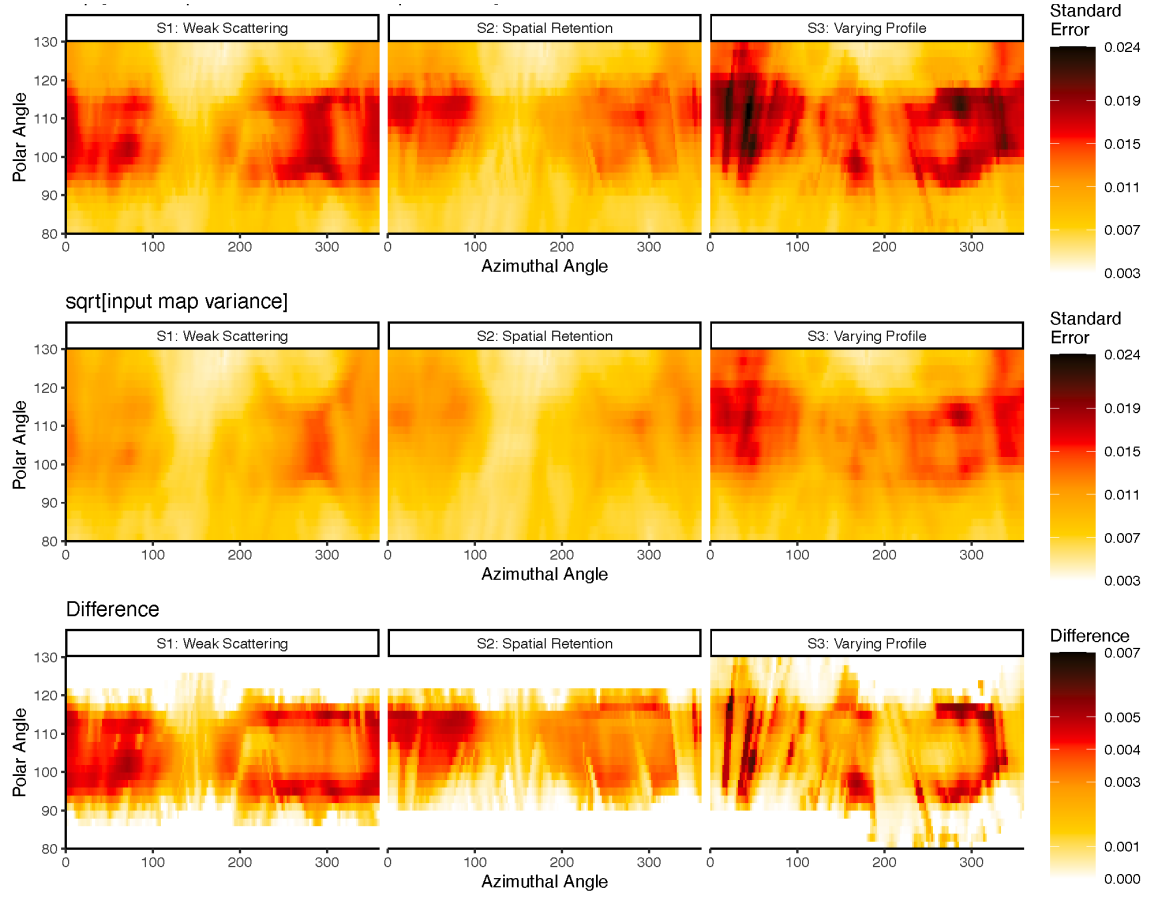

**Figure D5:** Skewness of the ribbon profiles in separated ribbon maps for each azimuthal sector

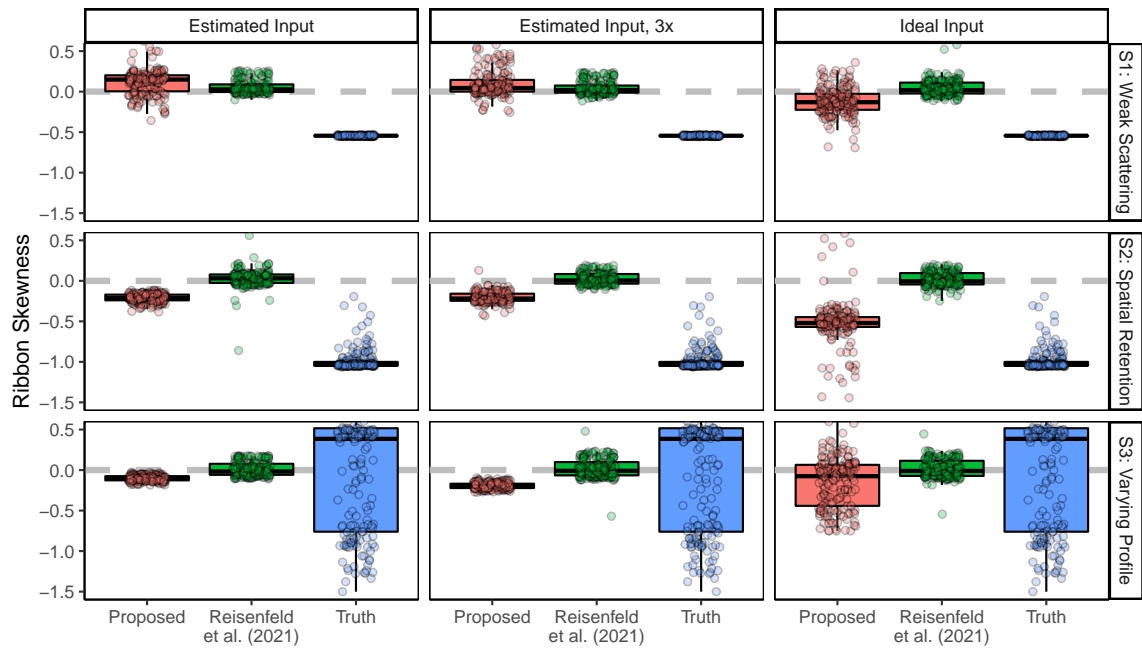

**Figure D6:** Width (measured by the full width at half-maximum) of the ribbon profiles in separated ribbon maps for each azimuthal sector

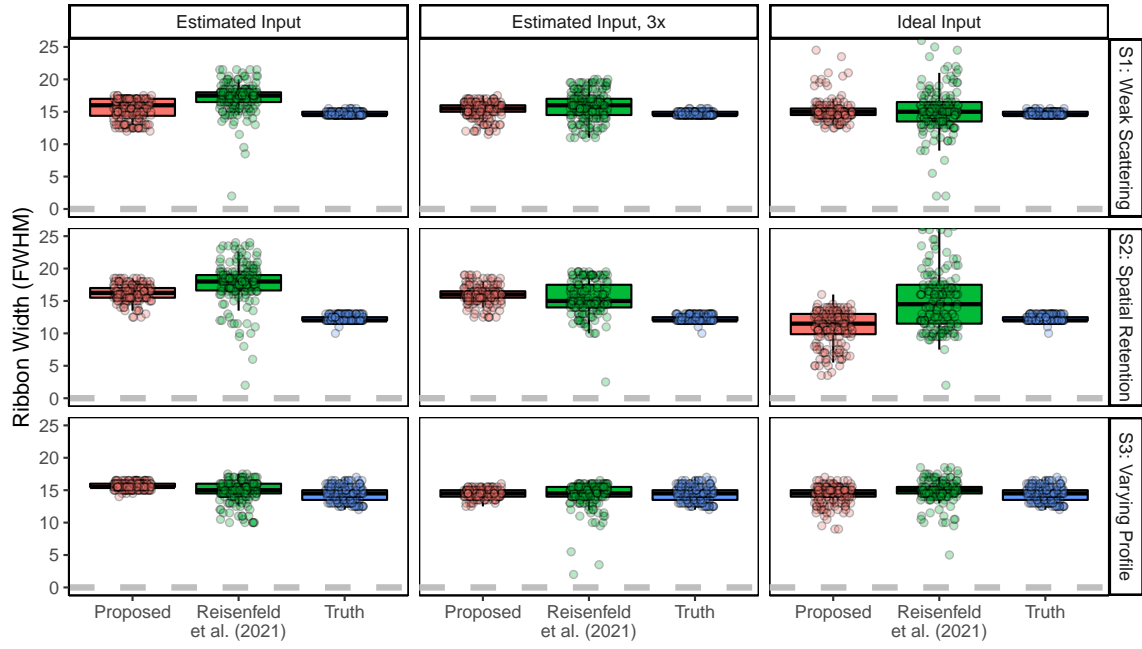

## E Ribbon Center Estimation in Simulated Data

In this section, we provide additional figures for the ribbon center estimation in simulated data.

First, we consider performance of the ribbon center estimation methods as a function of the number of pseudo-posterior draws used within the estimation algorithm. Estimation used the simulation truth ribbon-only maps. **Supp. Figure E1** shows the results. The method in Funsten et al. (2013) converges with few draws (e.g.,  $< 100$ ). The proposed method, which also draws the input map used for center estimation, requires more draws to reliably converge (e.g., 500). However, the practical difference in the point estimate between 100 and 500 draws for the proposed method is often negligible.

In practice, we may not always have a good estimate of the working rotational frame for estimation. If our initial working estimates are far from the truth (e.g., 2+ degrees in any direction), substantial bias can result. **Supp. Figure E2** illustrates bias in ribbon center estimation as a function of the working ribbon center (i.e., the working rotational frame) for the spatial retention simulation scenario using ribbon-only maps and performing only a single ribbon center estimation per map (i.e., no iteration). These results highlight that a poor working rotational frame can substantially impact bias in the final ribbon center estimate and that this bias is smaller for the proposed method. In general, ribbon center estimation using the weak scattering maps was less sensitive to the choice of the working ribbon center than the spatial retention or varying profile maps (results not shown).

Additional iterations of ribbon center estimation (i.e., the new ribbon center estimate becomes the new working rotational frame for the next iteration of estimation) can help reduce this bias substantially. **Supp. Figure E3** explores the bias in ribbon center estimates as a function of the number of iterations. Both the proposed method and the method in Funsten et al. (2013) produce essentially unbiased ribbon center estimates after several iterations for scenarios S1/S2. Both methods produce substantial bias for S3, and this bias tended to be higher for the proposed method.

**Figure E1:** Ribbon center latitude and longitude estimates as a function of the number of pseudo-posterior draws (lines) and corresponding 95% confidence interval estimates (shaded regions). Results based on simulation truth ribbon-only maps in the “correct” ribbon-centered rotational frame. In all scenarios, the true ribbon center was at longitude 221.5 and latitude 39.

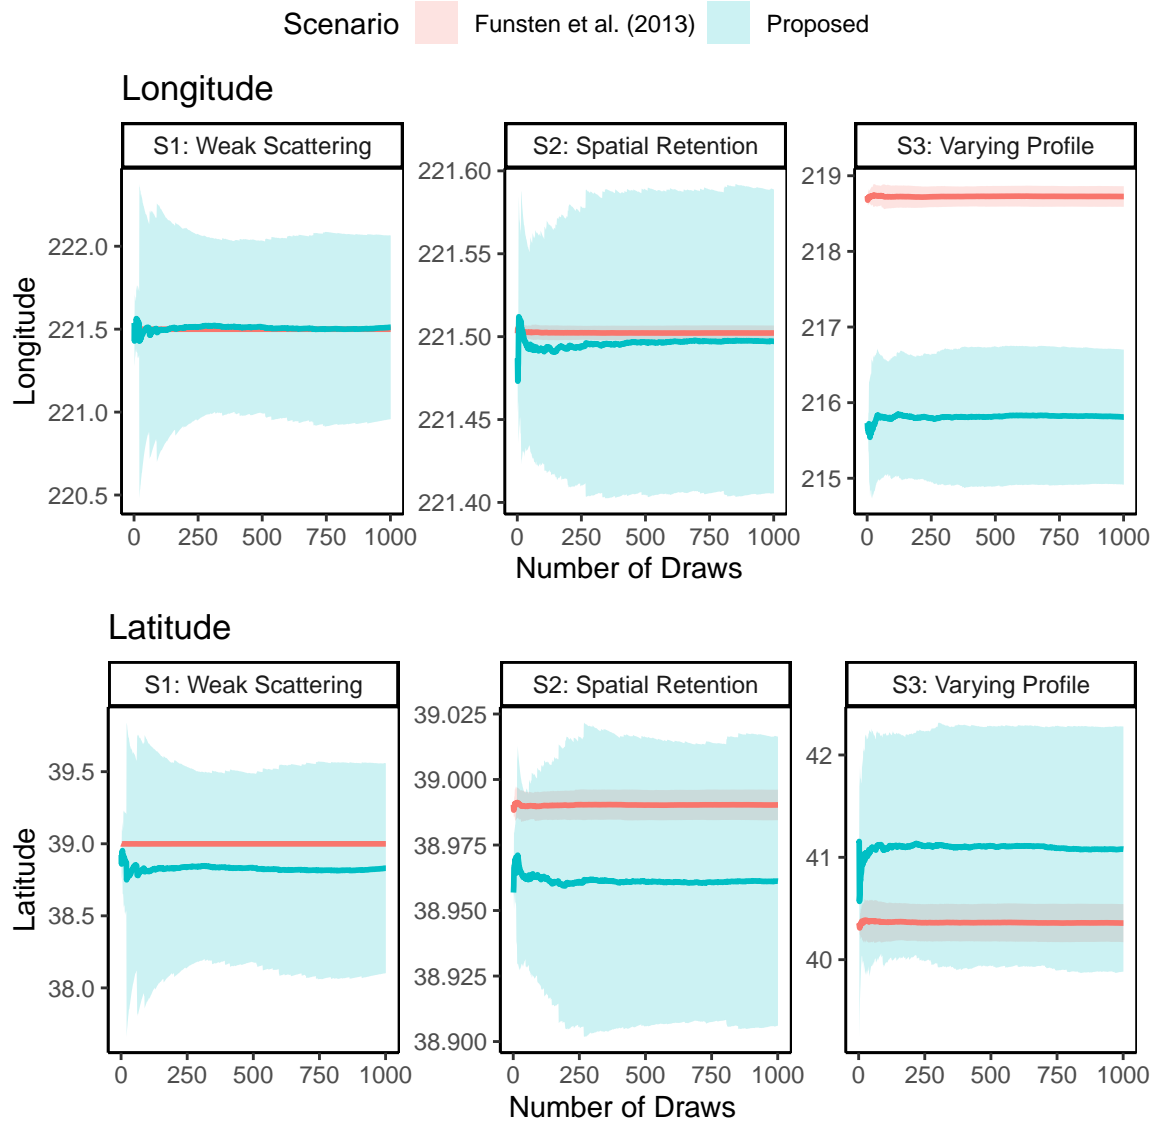

**Figure E2:** Distance between estimated and simulation true ribbon center (in degrees) as a function of the working ribbon center after a single iteration ribbon center estimation. The true ribbon center for these simulations is longitude 221.5 and latitude 39. Results are provided based on simulation truth ribbon only maps generated under simulation scenario S2 (i.e., spatial retention model).

|    | Funsten et al. (2013) |       |       |       |       |       |       | Proposed |       |       |       |       |       |       |                       |
|----|-----------------------|-------|-------|-------|-------|-------|-------|----------|-------|-------|-------|-------|-------|-------|-----------------------|
|    | 215.5                 | 217.5 | 219.5 | 221.5 | 223.5 | 225.5 | 227.5 | 215.5    | 217.5 | 219.5 | 221.5 | 223.5 | 225.5 | 227.5 |                       |
| 45 | 5.17                  | 3.19  | 2.6   | 1.34  | 1.84  | 2.03  | 2.45  | 0.55     | 0.64  | 0.77  | 0.68  | 0.5   | 0.57  | 1.16  | S2: Spatial Retention |
| 43 | 3.36                  | 1.65  | 0.88  | 0.51  | 0.5   | 1.1   | 1.84  | 0.4      | 0.37  | 0.48  | 0.69  | 0.45  | 0.95  | 0.96  |                       |
| 41 | 1.65                  | 0.55  | 0.28  | 0.18  | 0.24  | 0.54  | 1.73  | 0.44     | 0.21  | 0.27  | 0.24  | 0.5   | 1.16  | 0.99  |                       |
| 39 | 1.21                  | 0.42  | 0.16  | 0.01  | 0.16  | 0.42  | 1.18  | 0.33     | 0.22  | 0.05  | 0.04  | 0.08  | 0.77  | 0.85  |                       |
| 37 | 1.75                  | 0.54  | 0.24  | 0.16  | 0.28  | 0.59  | 1.75  | 0.45     | 0.21  | 0.08  | 0.08  | 0.27  | 0.51  | 0.79  |                       |
| 35 | 3.29                  | 1.23  | 0.61  | 0.48  | 0.76  | 1.63  | 3.9   | 0.41     | 0.1   | 0.08  | 0.11  | 0.29  | 0.48  | 0.58  |                       |
| 33 | 4.03                  | 3.38  | 2.42  | 2.48  | 3.16  | 4.11  | 3.87  | 0.41     | 0.19  | 0.15  | 0.26  | 0.4   | 0.45  | 0.56  |                       |

**Figure E3:** Impact of iteration on ribbon center estimates for “corner” working longitudes and latitudes in **Supp. Figure E2**. Results based on simulation truth ribbon-only maps. Lines correspond to estimated ribbon centers, and shaded regions correspond to 95% confidence intervals. Horizontal dashed lines indicate the simulation truths.

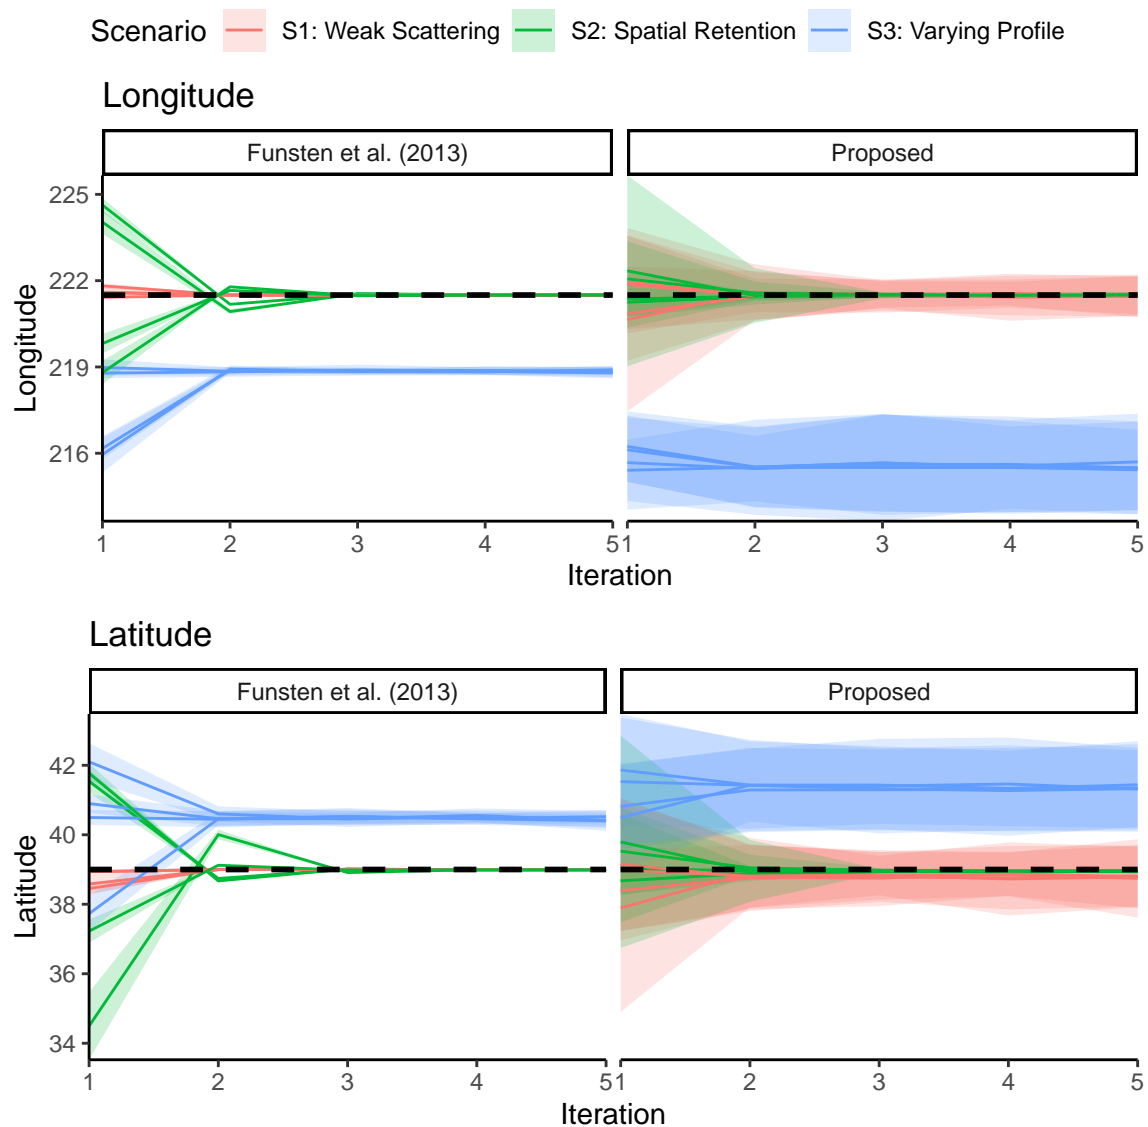

## F Additional results from real IBEX data analysis

Detailed results from the application of these methods to real data will be provided in follow-up papers. In this section, we provide limited additional results from these analyses. **Supp. Figure F1** shows cross-sections of the estimated ribbon maps using the proposed methods. Although our estimation algorithm did not borrow information across time, our separated maps demonstrate a gradually changing ribbon morphology, indicating that the proposed separation method is capturing “real” features observable in multiple maps.

**Supp. Figure F2** provides estimated GDF-only ram-only maps in ecliptic coordinates. For early years (e.g., 2009B-2010A), we can still see some potentially ribbon-like features in the ribbon region, even after separation. This may indicate imperfect ribbon separation (or input map estimation), or it may be “real,” and the observed data alone do not provide enough information to tell the difference. This is where subject-matter expertise will come in. For later years, there are no visible traces of the ribbon in the GDF maps, providing some evidence of high-quality ribbon separation.

**Figure F1:** Ribbon cross-sections for estimated ribbon-only 2-degree maps for energy step 4, ram direction. Results are shown in the ribbon-centric rotational frame for each map, where ribbon centers were re-estimated using each ribbon-only map. A/B maps correspond to the first and second 6-months of the year, respectively.

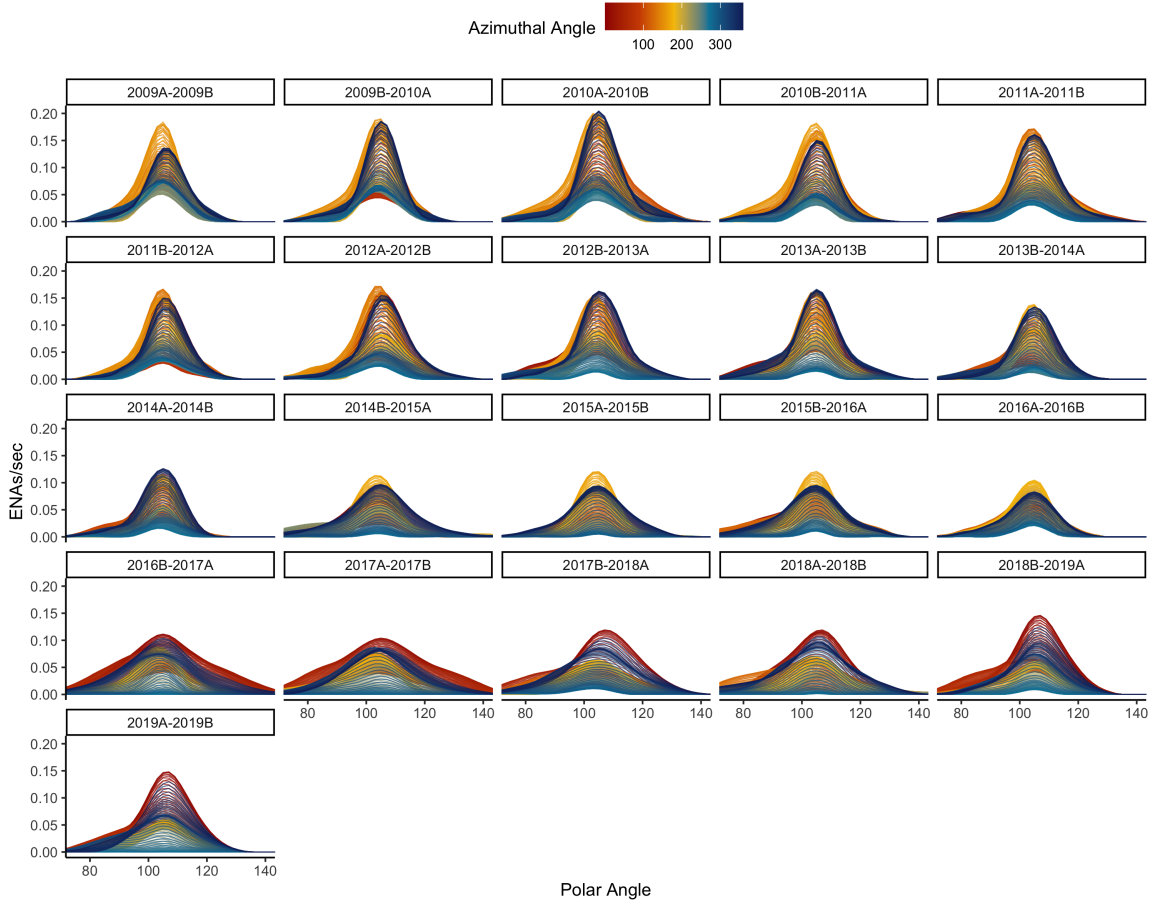

**Figure F2:** Ribbon-only and GDF-only maps for real IBEX 2-degree maps for energy step 4, ram direction in ecliptic coordinates. “Nose” and “tail” indicate the front and back of heliospheric bow shock, respectively. A/B maps correspond to the first and second 6-months of the year, respectively

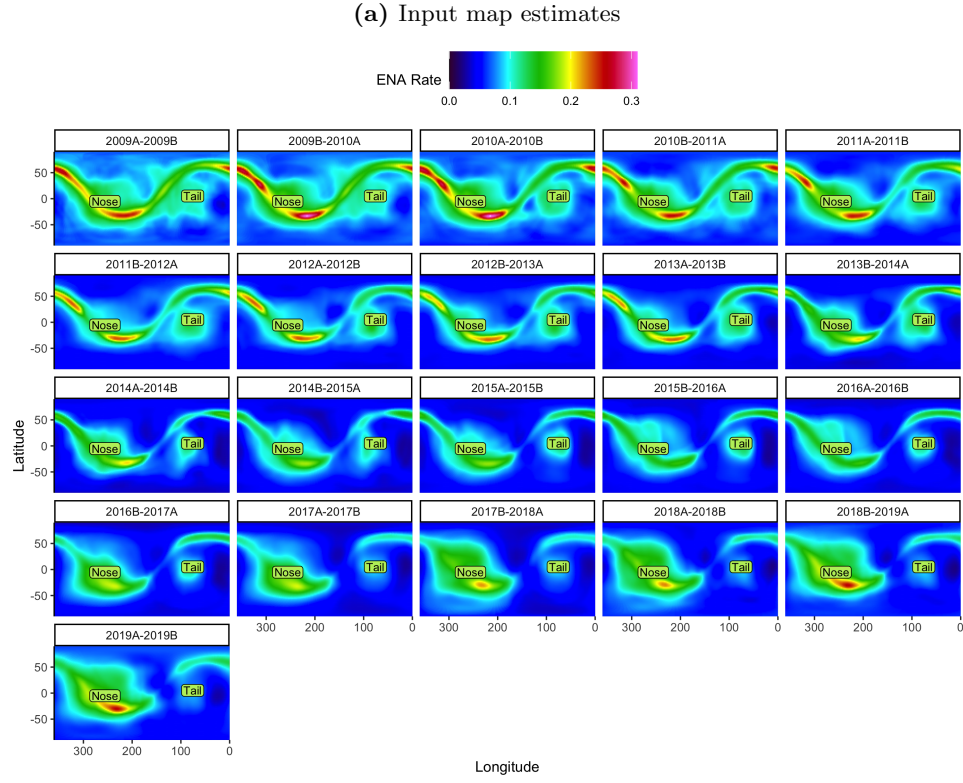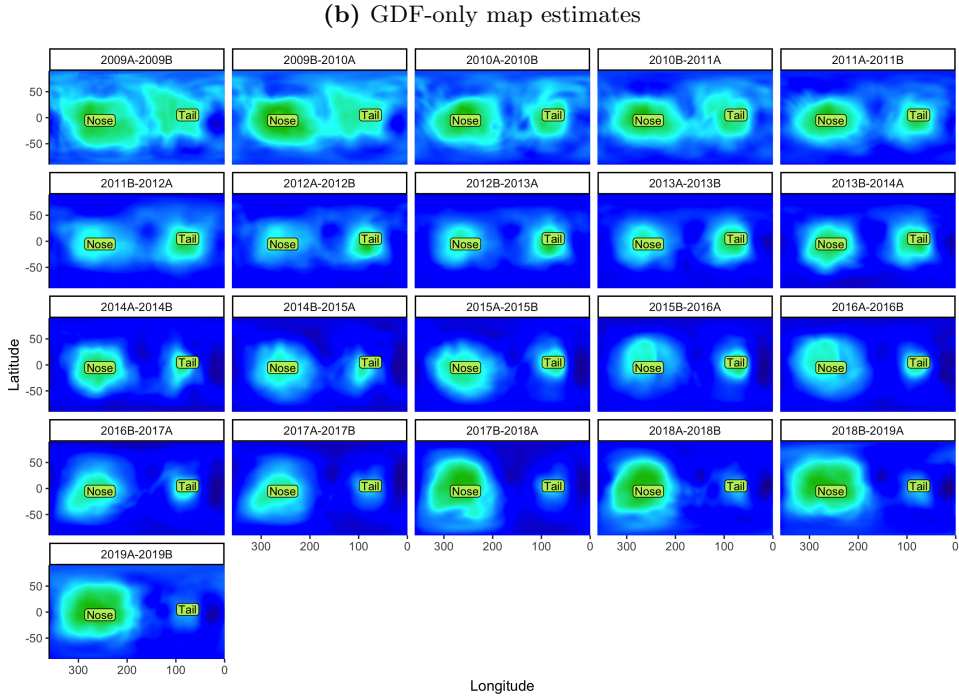

## G A note on empirical coverage and normality approximations

In this section, we put the empirical coverage results presented in the main paper in context by directly comparing these coverages to the coverages of the input total ENA rate maps. As shown in **Supp. Figure G1**, coverage of 95% confidence intervals for the estimated input maps were nearly always less than nominal. The coverage for the separated GDF map estimates is even lower. These results indicate that the under-coverage of the GDF-only maps obtained using the proposed method is a combination of (1) error in ribbon map separation and (2) under-coverage of the input maps in the ribbon region.

An alternative explanation for under-coverage could be inadequacy of the normal distribution assumptions made in the course of uncertainty estimation. As a simple evaluation of this assumption, we consider the input map estimates and their corresponding uncertainties. We compare 95% confidence intervals obtained for these point estimates using normal distributional assumptions with 2.5% and 97.5% quantiles of the input map estimates obtained automatically via bootstrap in Osthus et al. (2022). These latter quantiles were obtained without assuming normality of the ENA rates. If the two sets of constructed confidence intervals are very similar, this provides some evidence of the reasonableness of the normality assumption for confidence interval construction.

**Supp. Figure G2** provides this comparison. We observe very strong correspondence between the confidence intervals constructed under the two methods, both in terms of the confidence interval widths and the individual upper and lower bounds. One exception is the scenario where confidence intervals are very wide relative to the magnitude of the point estimate, usually due to ENA rates very near zero. For these pixels, the normal approximation results in confidence intervals that are slightly shifted away from zero, relative to the quantile-based confidence intervals. Still, this difference is minimal and primarily located away from the ribbon region, suggesting that normal distribution approximations may be reasonable for ribbon separation-related uncertainties.

**Figure G1:** Coverage of 95% confidence intervals for the input total ENA rate map estimates and the separated GDF-only maps in the ribbon region. Separated maps were obtained using the proposed method and the method in Reisenfeld et al. (2021). All confidence intervals were calculated using normal distribution approximations, i.e., estimate  $\pm 1.96\sqrt{\text{variance estimate}}$ . Within each panel and row, the highest coverage proportion is highlighted.

|                       | Estimated Input            |             |                             | Estimated Input, 3x        |             |                             | Ideal Input                |          |                             |
|-----------------------|----------------------------|-------------|-----------------------------|----------------------------|-------------|-----------------------------|----------------------------|----------|-----------------------------|
| S1: Weak Scattering   | <b>0.98</b>                | 0.94        | 0.84                        | <b>0.91</b>                | 0.84        | 0.66                        | <b>1</b>                   | 0.98     | 0.87                        |
| S2: Spatial Retention | 0.88                       | <b>0.88</b> | 0.85                        | <b>0.87</b>                | 0.8         | 0.72                        | <b>1</b>                   | 1        | 0.81                        |
| S3: Varying Profile   | <b>0.83</b>                | 0.7         | 0.71                        | 0.78                       | <b>0.83</b> | 0.68                        | <b>1</b>                   | 0.86     | 0.76                        |
|                       | Benchmark<br>Total ENA Map | Proposed    | Reisenfeld<br>et al. (2021) | Benchmark<br>Total ENA Map | Proposed    | Reisenfeld<br>et al. (2021) | Benchmark<br>Total ENA Map | Proposed | Reisenfeld<br>et al. (2021) |

**Figure G2:** Comparison of 95% confidence interval bounds and widths obtained for input ENA rate maps based on normal distribution approximations vs. using bootstrap estimate quantiles. Points correspond to each of 16200 pixels across 8 simulated maps generated using the method in Osthus et al. (2022)

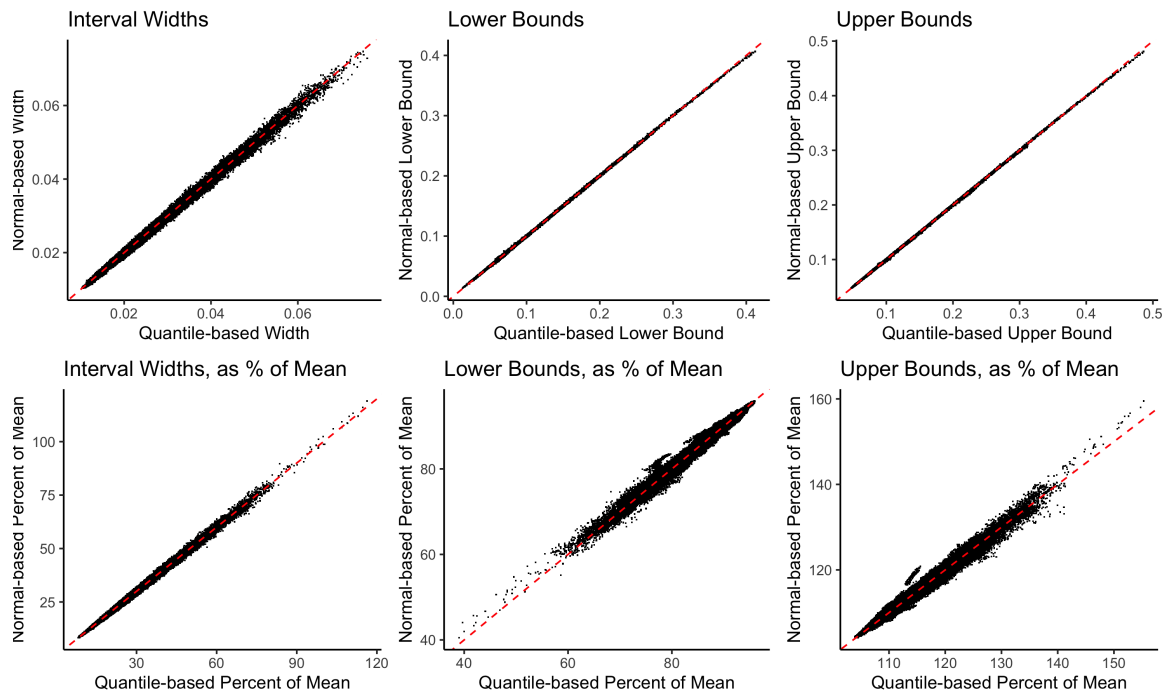

## H Choosing mask tuning parameters

Within our ribbon mask framework, the mask formulation may depend on the specification of two tuning parameters: (1) the ribbon bounds (i.e., the distance from the peak defining all pixels that could contain non-negligible ribbon flux) and (2) the threshold of Sobel filter values (in terms of quantiles within the ribbon bound region) used to identify the edges of the ribbon. Small values of (1) and/or large values of (2) may result in masks that are too narrow, while large values of (1) and/or small values of (2) may result in masks that contain the ribbon but are too wide to be useful. The impact of these tuning parameter choices on simulated map separations is summarized in terms of the mean absolute percent error in GDF estimates (relative to simulation truths) in the ribbon region in **Supp. Figure H1**. Within each panel, circles denote the optimal value, and stars indicate the combination of 30 degrees bound and a quantile threshold of 0.75 for visual comparison. The absolute percent error is clearly sensitive to the tuning parameter choice.

Therefore, we propose repeating our analysis across a grid of values and defining some metric for determining the “best” combination of tuning parameters for a given map. The “best” combination may sometimes be apparent to the trained eye upon visual inspection of the ribbon separations, but practical implementation of eyeball-based sensitivity analysis is cumbersome and subjective. Therefore, we propose data-driven metrics for determining which combinations of input parameters are “best” among several candidates. For real data applications, we restrict our sensitivity analyses to ribbon bounds of at least 30 degrees, since narrower ribbon bounds often under-performed.

**Figure H1:** Comparison of mean absolute percent error in GDF map estimates, relative to simulation truths, as a function of mask tuning parameters. Within each panel, circles denote the optimal value, and stars indicate the combination of 30 degrees bound and a quantile threshold of 0.75 for visual comparison.

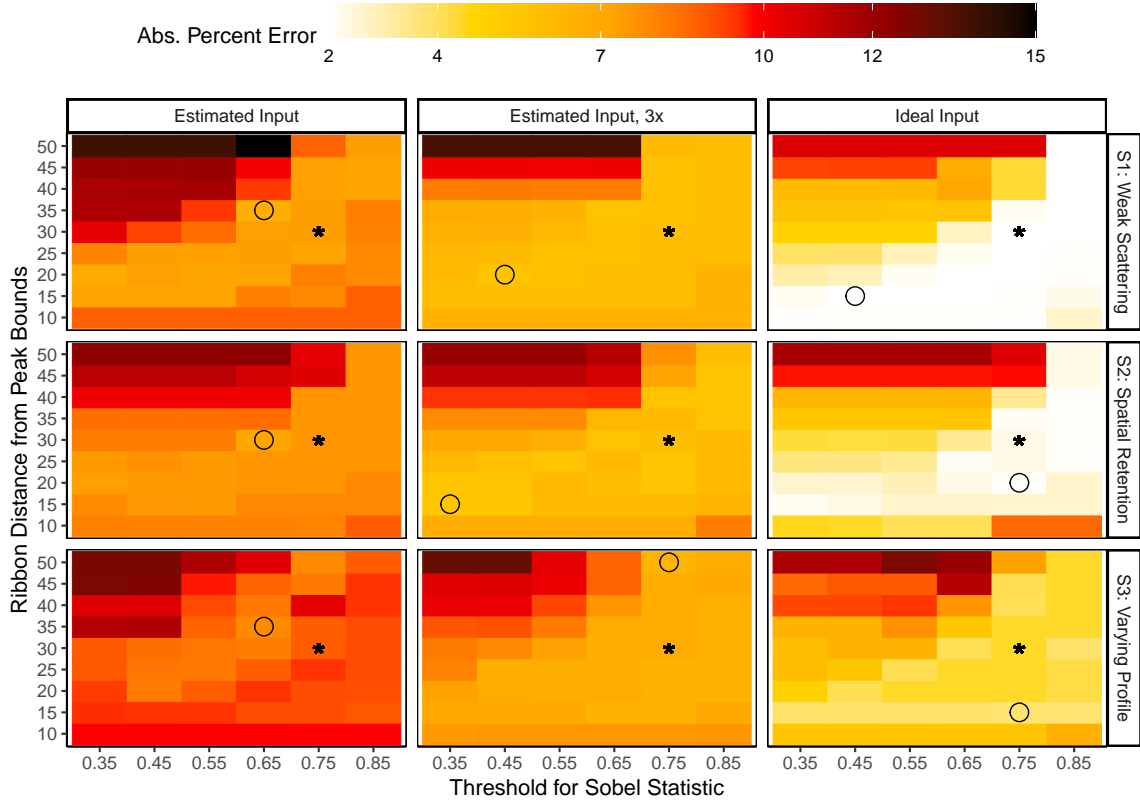

## H.1 Proposed sensitivity analysis metrics

For simulated datasets, it is straightforward to determine the “best” values of the tuning parameters based on the map separation accuracy, coverage, etc. However, our goal is to develop and implement metrics that can be used to evaluate the ribbon separations for real data. We therefore return to the thorny problem of quantifying what makes a “good” ribbon separation.

Of course, we can calculate various summary metrics characterizing ribbon morphology, including peak height, width, skewness, kurtosis, etc. However, it can be difficult to use these metrics alone to optimize tuning parameter choice. Instead, we turn to another theoretical property of the maps: on average, we expect the estimated ribbon and GDF maps to have low correlation. That is, across the entire map or a large sub-section, we do not expect the ribbon and GDF to co-vary; negative correlations are particularly troubling. We emphasize that this is a global map property, and local regions of the ribbon and GDF map estimates will often have non-zero correlation. We propose calculating the correlation between the estimated GDF and ribbon maps, restricted to the mask region with non-zero estimated ribbon. This final restriction avoids biasing these correlation estimates toward maps with little non-zero ribbon flux. **Supp. Figure H2** shows the relationship between this estimated correlation and the average percent error for the simulated data maps. The red plotted points correspond to the combination of 30 degrees and a quantile threshold of 0.75. We find that there is an association between the estimation accuracy and the ribbon/GDF correlation. However, the strength of this association varies from map to map, and the point with the correlation value closest to zero may not always correspond to a tuning parameter combination with low GDF map estimation error.

In light of the potential under-performance of the ribbon/GDF correlation alone in discriminating good/bad tuning parameter choices, we propose an additional metric for measuring the separation performance. Another feature of a “good” map separation is that it results in GDF estimates that are fairly slowly-varying in space; large local changes in GDF flux in the ribbon region of the GDF-only map can be an indicator of either (1) missed edges of the ribbon (suggesting our mask was too narrow) or (2) missing GDF flux that should be present (suggesting our mask was too large/the ribbon separation took too much). In either case, we propose applying the Sobel edge detection methodology to the GDF map estimate and comparing the “edge-iness” across tuning parameter specifications. In **Supp. Figure H3**, we illustrate the results of applying the Sobel filter to the GDF map estimate for the Simulation Scenario S1 (Weak Scattering) obtained using ideal ribbon separation inputs. In all Sobel maps, we can see evidence of horizontal banding, indicative of imperfect ribbon separation. However, some Sobel maps have more bandedness than others, indicating worse performance. In practice, we propose summarizing the relative bandedness of each Sobel map as follows:

1. For each pixel, subtract the median Sobel metric value for that pixel across all candidate tuning parameter combinations. This allows us to focus our attention on pixels with varying Sobel metrics between separated maps. We will call this resulting map the Sobel “deviation” map.
2. For each map, calculate the sum of squared Sobel deviation map values across all pixels.

The resulting metric can be used to summarize the map separation, where lower values are often associated with better map separations.

Although not shown in detail, each of these metrics (Sobel-based metric and correlation of ribbon and GDF maps) does an imperfect job of identifying the best map separation among many candidates. However, their combined information can do a decent job of discrimination, as illustrated in **Supp. Figure H4**. We ultimately propose defining the best tuning parameter value as the combination that minimizes the sum of the squared correlation and the squared

**Figure H2:** Relationship between GDF map average percent estimation error and the correlation between the GDF and ribbon map estimates as a function of mask tuning parameters. Red plotted points indicate the combination of 30 degrees bound and a quantile threshold of 0.75 for visual comparison. Correlations were calculated restricting to map pixels with non-zero ribbon flux in the estimated ribbon map.

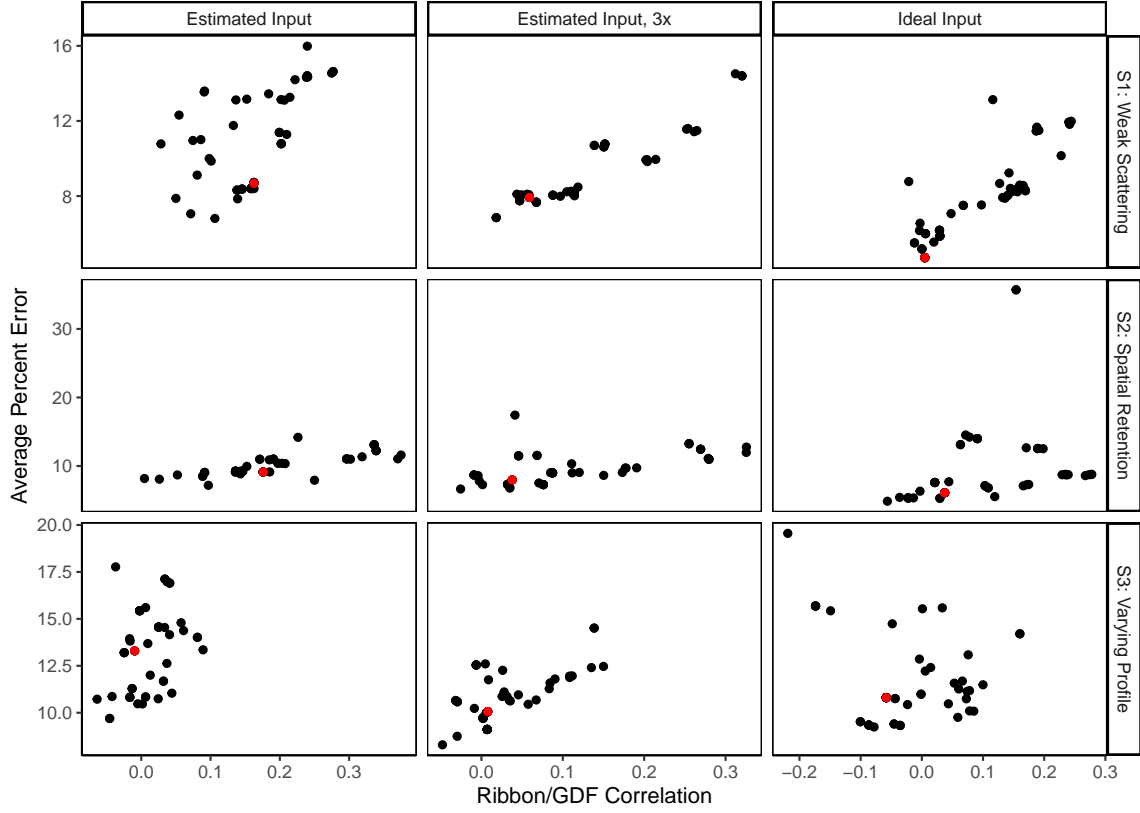

Sobel metric (scaled by its maximum value across tuning parameter values). In practice, we restrict our chosen parameter values to those with ribbon bounds equal to or greater than 30. The resulting tuning parameter combination is similar to or better than results using bounds = 30, threshold = 0.75 for all maps except scenario S3: Varying Profile with 1x estimated input maps. For this map, the “optimal” value resulted in a decrease in GDF map accuracy of roughly 3% in the ribbon region.

**Figure H3:** Results of applying to Sobel filter to estimated GDF-only maps obtained by applying the proposed ribbon separation methodology to ideal (simulation truth) S1: Weak Scattering maps. Results shown fixing the threshold tuning parameter to 0.75.

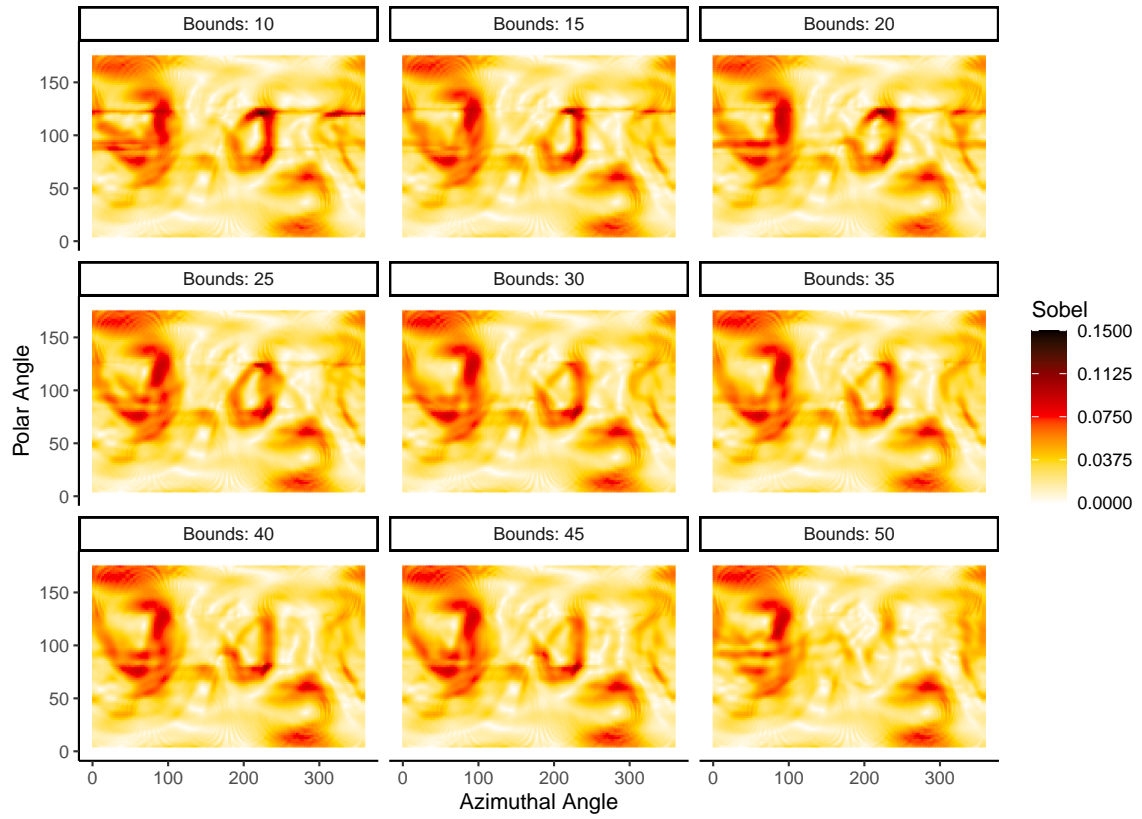

**Figure H4:** Relationships between average absolute percent error in GDF map estimates, (1) correlation between ribbon and GDF map estimates in the ribbon region, and (2) Sobel sum of squared deviations metric, calculated across the entire GDF map.

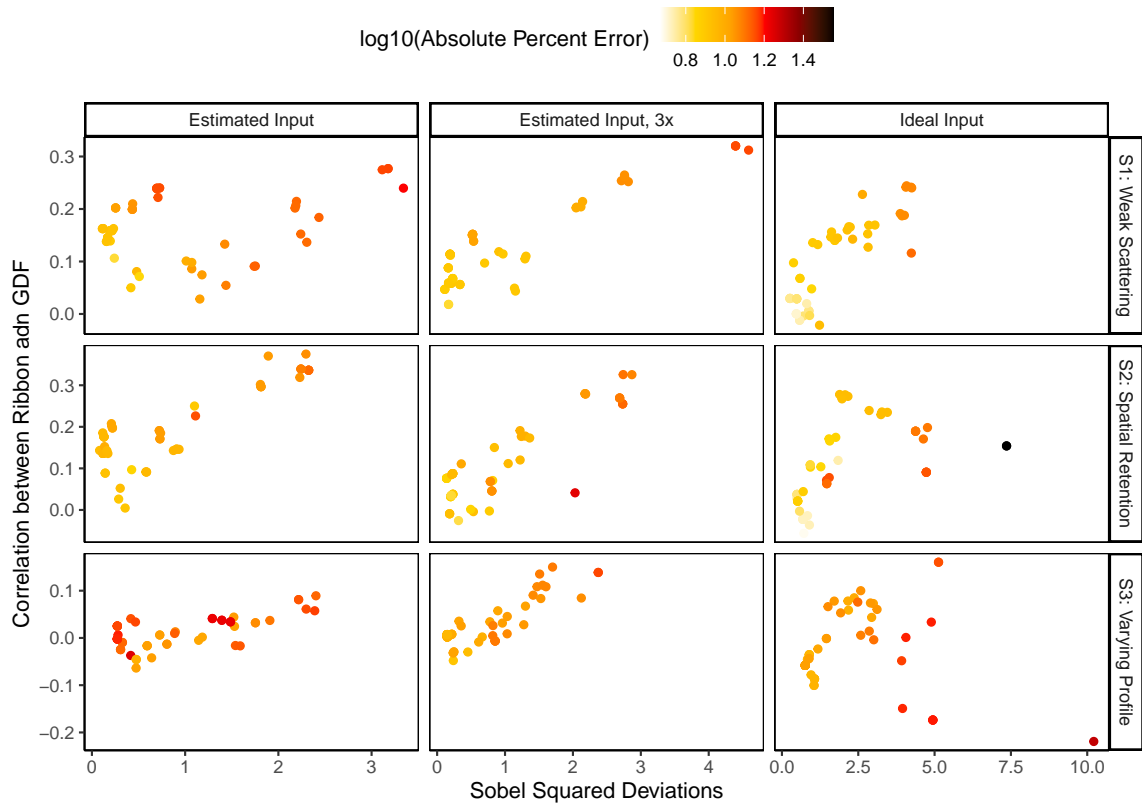

## References

- Avrim Blum, John Hopcroft, and Ravindran Kannan. *Foundations of Data Science*. Cambridge University Press, 2015.
- Jian S Dai. Euler–rodrigues formula variations, quaternion conjugation and intrinsic connections. *Mechanism and Machine Theory*, 92:144–152, 2015.
- B Efron and C Stein. The jackknife estimate of variance. *The Annals of Statistics*, 9:586–596, 1981.
- Andrew Fitzgibbon, Maurizio Pilu, and Robert B. Fisher. Direct least square fitting of ellipses. *IEEE Transactions on Pattern Analysis and Machine Intelligence*, 21:476–480, 1999. ISSN 01628828. doi: 10.1109/34.765658.
- H. O. Funsten, R. Demajistre, P. C. Frisch, J. Heerikhuisen, D. M. Higdon, P. Janzen, B. A. Larsen, G. Livadiotis, D. J. McComas, E. Möbius, C. S. Reese, D. B. Reisenfeld, N. A. Schwadron, and E. J. Zirnstein. Circularity of the interstellar boundary explorer ribbon of enhanced energetic neutral atom (ena) flux. *Astrophysical Journal*, 776, 10 2013. ISSN 15384357. doi: 10.1088/0004-637X/776/1/30.
- Rob J Hyndman and Yeasmin Khandakar. Automatic time series forecasting: the forecast package for R. *Journal of Statistical Software*, 26(3):1–22, 2008. doi: 10.18637/jss.v027.i03.
- Dave Osthus, Brian P. Weaver, Lauren J. Beesley, Kelly R. Moran, Madeline A. Ausdemore, Eric J. Zirnstein, Paul H. Janzen, and Daniel B. Reisenfeld. Towards improved heliosphere sky map estimation with theseus, 2022. URL <https://arxiv.org/abs/2210.12005>.
- J. O. Ramsay. Monotone regression splines in action. *Statistical Science*, 3, 1988. ISSN 08834237. doi: 10.1214/ss/1177012761.
- Daniel B. Reisenfeld, Maciej Bzowski, Herbert O. Funsten, Jacob Heerikhuisen, Paul H. Janzen, Marzena A. Kubiak, David J. McComas, Nathan A. Schwadron, Justyna M. Sokół, Alex Zimorino, and Eric J. Zirnstein. A three-dimensional map of the heliosphere from ibex. *The Astrophysical Journal Supplement Series*, 254:40, 6 2021. ISSN 0067-0049. doi: 10.3847/1538-4365/abf658.
